# Supplementary material for: Renormalized Singles with Correlation in $GW$ Green's Function Theory for Accurate Quasiparticle Energies
Source: arXiv:2207.06520 ancillary file (2022-07-13)
Supplement: Supplementary file 1 [file supporting_information.pdf]

# Supporting Information: Renormalized Singles with Correlation in $GW$ Green's Function Theory for Accurate Quasiparticle Energies

Jiachen Li and Weitao Yang*

*Department of Chemistry, Duke University, Durham, NC 27708, USA*

E-mail: weitao.yang@duke.edu

## 1 RS Green's Function

To use the form of the HF self-energy to eliminate the starting point dependence, the RS Green's function is defined as

$$G_{\mathrm{RS}}^{-1} = G_0^{-1} - P(\Sigma_{\mathrm{Hx}}[G_0] - v_{\mathrm{Hxc}})P - Q(\Sigma_{\mathrm{Hx}}[G_0] - v_{\mathrm{Hxc}})Q, \tag{1}$$

where $P = \sum_i^{occ} |\psi_i^{(0)}\rangle\langle\psi_i^{(0)}|$ is the projection into the occupied orbital space and $Q = I - P$ is the projection into the virtual orbital space, $\Sigma_{\mathrm{Hx}}[G_0]$ means that the HF (Hartree and exchange) self-energy is constructed with the KS Green's function, $\{\psi^0\}$ are KS orbitals. We use $i$, $j$ for occupied orbitals, $a$, $b$ for virtual orbitals, $p$, $q$ for general orbitals.

Equivalently, the RS Green's function is obtained by using the KS density matrix in the HF Hamiltonian, which is the RS Hamiltonian $H^{\mathrm{RS}} = H^{\mathrm{HF}}[G_0]$, and solving two projected HF equa-

tions in the occupied subspace and the virtual subspaces[S1]

$$P(H^{\mathrm{HF}}[G_0])P|\psi_i^{\mathrm{RS}}\rangle = P(H^{\mathrm{RS}})P|\psi_i^{\mathrm{RS}}\rangle = \epsilon_i^{\mathrm{RS}} P|\psi_i^{\mathrm{RS}}\rangle, \tag{2}$$

and

$$Q(H^{\mathrm{HF}}[G_0])Q|\psi_a^{\mathrm{RS}}\rangle = Q(H^{\mathrm{RS}})Q|\psi_i^{\mathrm{RS}}\rangle = \epsilon_a^{\mathrm{RS}} Q|\psi_a^{\mathrm{RS}}\rangle. \tag{3}$$

# 2 Ionization Potentials of the GW100 Set Obtained from Different *GW* Methods

**Table S1:** Ionization potentials of the GW100 set[S2] obtained from $G_0W_0$ with HF, BLYP, PBE, B3LYP and PBE0. The def2-TZVPP basis set was used. Systems containing Xe, Rb, I, Ag and Cu were excluded because of the convergence problem. All values in eV.

| | | | $G_0W_0$ | | | | |
|---|---|---|---|---|---|---|---|
| name | formula | Exp | HF | BLYP | PBE | B3LYP | PBE0 |
| helium | He | 24.59 | 24.60 | 23.80 | 23.84 | 24.06 | 24.12 |
| neon | Ne | 21.56 | 21.41 | 20.54 | 20.57 | 20.79 | 20.85 |
| argon | Ar | 15.76 | 15.73 | 15.05 | 15.05 | 15.22 | 15.25 |
| krypton | Kr | 14.00 | 13.96 | 13.36 | 13.35 | 13.50 | 13.52 |
| hydrogen | $H_2$ | 15.43 | 16.49 | 15.93 | 15.96 | 16.14 | 16.19 |
| lithium dimer | $Li_2$ | 4.73 | 5.29 | 5.02 | 5.08 | 5.17 | 5.22 |
| sodium dimer | $Na_2$ | 4.89 | 4.95 | 4.85 | 4.88 | 4.94 | 4.95 |
| sodium tetramer | $Na_4$ | 4.27 | 4.26 | 4.05 | 4.11 | 4.17 | 4.20 |
| sodium hexamer | $Na_6$ | 4.12 | 4.43 | 4.20 | 4.23 | 4.30 | 4.32 |
| potassium dimer | $K_2$ | 4.06 | 4.05 | 3.94 | 3.95 | 4.02 | 4.01 |
| nitrogen | $N_2$ | 15.58 | 17.10 | 14.80 | 14.85 | 15.20 | 15.31 |
| phosphorus dimer | $P_2$ | 10.62 | 10.52 | 10.05 | 10.07 | 10.19 | 10.22 |
| arsenic dimer | $As_2$ | 10.00 | 6.31 | 9.28 | 9.30 | 9.39 | 9.41 |
| fluorine | $F_2$ | 15.70 | 16.32 | 14.91 | 14.96 | 15.30 | 15.41 |
| chlorine | $Cl_2$ | 11.49 | 11.75 | 10.95 | 10.97 | 11.16 | 11.20 |
| bromine | $Br_2$ | 10.51 | 10.71 | 9.97 | 9.98 | 10.15 | 10.18 |
| methane | $CH_4$ | 14.35 | 14.75 | 13.94 | 13.93 | 14.17 | 14.19 |

**Table S1:** Continued

| name | formula | Exp | $G_0W_0$ | | | | |
|---|---|---|---|---|---|---|---|
| | | | HF | BLYP | PBE | B3LYP | PBE0 |
| ethane | $C_2H_6$ | 12.20 | 13.16 | 12.36 | 12.35 | 12.58 | 12.59 |
| propane | $C_3H_8$ | 11.51 | 12.60 | 11.80 | 11.77 | 12.02 | 12.02 |
| butane | $C_4H_{10}$ | 11.09 | 12.15 | 11.50 | 11.47 | 11.72 | 11.72 |
| ethylene | $C_2H_4$ | 10.68 | 10.73 | 10.26 | 10.26 | 10.40 | 10.41 |
| ethyn | $C_2H_2$ | 11.49 | 11.56 | 10.96 | 10.97 | 11.13 | 11.16 |
| tetracarbon | $C_4$ | 12.54 | 11.59 | 10.68 | 10.72 | 10.99 | 11.06 |
| cyclopropane | $C_3H_6$ | 10.54 | 11.26 | 10.48 | 10.47 | 10.68 | 10.69 |
| benzene | $C_6H_6$ | 9.23 | 9.48 | 8.89 | 8.89 | 9.06 | 9.07 |
| cyclooctatetraene | $C_8H_8$ | 8.43 | 8.64 | 7.96 | 7.95 | 8.15 | 8.15 |
| cyclopentadiene | $C_5H_6$ | 8.53 | 8.82 | 8.26 | 8.25 | 8.43 | 8.43 |
| vinyl fluoride | $C_2H_3F$ | 10.63 | 10.80 | 10.09 | 10.09 | 10.29 | 10.30 |
| vinyl chloride | $C_2H_3Cl$ | 10.20 | 10.34 | 9.64 | 9.64 | 9.83 | 9.85 |
| vinyl bromide | $C_2H_3Br$ | 9.90 | 9.42 | 8.83 | 8.82 | 8.99 | 8.99 |
| tetrafluoromethane | $CF_4$ | 16.20 | 16.84 | 15.25 | 15.29 | 15.71 | 15.82 |
| tetrachloromethane | $CCl_4$ | 11.69 | 11.97 | 10.86 | 10.86 | 11.17 | 11.22 |
| tetrabromomethane | $CBr_4$ | 10.54 | 10.72 | 9.69 | 9.69 | 9.97 | 10.00 |
| silane | $SiH_4$ | 12.82 | 13.22 | 12.33 | 12.33 | 12.61 | 12.64 |
| germane | $GeH_4$ | 12.46 | 12.85 | 12.03 | 12.03 | 12.26 | 12.29 |
| disilane | $Si_2H_6$ | 10.53 | 11.07 | 10.27 | 10.22 | 10.48 | 10.46 |
| pentasilane | $Si_5H_{12}$ | 9.36 | 9.77 | 8.88 | 8.82 | 9.11 | 9.07 |
| lithium hydride | LiH | 7.90 | 8.15 | 6.93 | 7.03 | 7.49 | 7.61 |
| potassium hydride | KH | 8.00 | 6.29 | 5.03 | 5.08 | 5.55 | 5.65 |
| borane | $BH_3$ | 12.03 | 13.65 | 12.88 | 12.89 | 13.13 | 13.16 |
| diborane | $B_2H_6$ | 11.90 | 12.79 | 11.86 | 11.84 | 12.13 | 12.15 |
| ammonia | $NH_3$ | 10.82 | 11.17 | 10.29 | 10.33 | 10.53 | 10.59 |
| hydrazoic acid | $HN_3$ | 10.72 | 11.06 | 10.24 | 10.28 | 10.47 | 10.53 |
| phosphine | $PH_3$ | 10.59 | 10.77 | 10.23 | 10.21 | 10.38 | 10.38 |
| arsine | $AsH_3$ | 10.58 | 10.55 | 10.08 | 10.05 | 10.19 | 10.18 |
| hydrogen sulfide | $SH_2$ | 10.50 | 10.49 | 9.94 | 9.93 | 10.08 | 10.09 |
| hydrogen fluoride | FH | 16.12 | 16.21 | 15.30 | 15.35 | 15.56 | 15.64 |
| hydrogen chloride | ClH | 12.79 | 12.78 | 12.15 | 12.15 | 12.31 | 12.33 |
| lithium fluoride | LiF | 11.30 | 11.34 | 10.05 | 10.09 | 10.57 | 10.66 |

**Table S1:** Continued

| name | formula | Exp | $G_0W_0$ | | | | |
|---|---|---|---|---|---|---|---|
| | | | HF | BLYP | PBE | B3LYP | PBE0 |
| magnesium fluoride | $F_2Mg$ | 13.30 | 13.82 | 12.43 | 12.48 | 12.96 | 13.07 |
| titanium tetrafluoride | $TiF_4$ | | 16.06 | 13.88 | 13.92 | 14.57 | 14.72 |
| aluminum fluoride | $AlF_3$ | 15.45 | 15.61 | 14.18 | 14.24 | 14.66 | 14.78 |
| boron monofluoride | BF | 11.00 | 11.30 | 10.48 | 10.51 | 10.77 | 10.83 |
| sulfur tetrafluoride | $SF_4$ | 12.00 | 13.30 | 11.97 | 11.97 | 12.33 | 12.36 |
| potassium bromide | BrK | 8.82 | 8.18 | 7.38 | 7.43 | 7.68 | 7.73 |
| gallium monochloride | GaCl | 10.07 | 9.90 | 9.42 | 9.43 | 9.55 | 9.57 |
| sodium chloride | NaCl | 9.80 | 9.20 | 8.24 | 8.28 | 8.62 | 8.68 |
| magnesium chloride | $MgCl_2$ | 11.80 | 11.88 | 10.94 | 10.97 | 11.24 | 11.31 |
| boron nitride | BN | | 11.71 | 10.68 | 10.84 | 11.36 | 11.44 |
| hydrogen cyanide | NCH | 13.61 | 13.85 | 13.13 | 13.16 | 13.35 | 13.40 |
| phosphorus mononitr | PN | 11.88 | 12.34 | 11.03 | 11.12 | 11.42 | 11.56 |
| hydrazine | $H_2NNH_2$ | 8.98 | 10.14 | 9.22 | 9.25 | 9.46 | 9.52 |
| formaldehyde | $H_2CO$ | 10.89 | 11.34 | 10.25 | 10.31 | 10.56 | 10.65 |
| methanol | $CH_4O$ | 10.96 | 11.54 | 10.47 | 10.51 | 10.75 | 10.83 |
| ethanol | $C_2H_6O$ | 10.64 | 11.26 | 10.08 | 10.11 | 10.38 | 10.46 |
| acetaldehyde | $C_2H_4O$ | 10.24 | 10.78 | 9.50 | 9.54 | 9.87 | 9.95 |
| ethoxy ethane | $C_4H_{10}O$ | 9.61 | 10.46 | 9.23 | 9.27 | 9.55 | 9.64 |
| formic acid | $CH_2O_2$ | 11.50 | 11.92 | 10.66 | 10.71 | 11.04 | 11.14 |
| hydrogen peroxide | HOOH | 11.70 | 12.04 | 10.88 | 10.94 | 11.20 | 11.30 |
| water | $H_2O$ | 12.62 | 12.85 | 11.93 | 11.98 | 12.18 | 12.26 |
| carbon dioxide | $CO_2$ | 13.77 | 14.20 | 13.07 | 13.14 | 13.39 | 13.49 |
| carbon disulfide | $CS_2$ | 10.09 | 10.29 | 9.58 | 9.61 | 9.78 | 9.81 |
| carbon oxide sulfide | OCS | 11.19 | 11.52 | 10.75 | 10.77 | 10.96 | 11.00 |
| carbon oxide selenide | OCSe | 10.37 | 10.66 | 9.99 | 10.00 | 10.17 | 10.19 |
| carbon monoxide | CO | 14.01 | 15.04 | 13.51 | 13.54 | 13.92 | 14.02 |
| ozone | $O_3$ | 12.73 | 13.52 | 11.80 | 11.84 | 12.33 | 12.45 |
| sulfur dioxide | $SO_2$ | 12.50 | 12.94 | 11.67 | 11.71 | 12.00 | 12.08 |
| beryllium monoxide | BeO | 10.10 | 9.78 | 9.19 | 9.26 | 9.48 | 9.55 |
| magnesium monoxide | MgO | 8.76 | 8.40 | 6.94 | 6.96 | 7.35 | 7.37 |
| toluene | $C_7H_8$ | 8.82 | 9.11 | 8.52 | 8.51 | 8.69 | 8.69 |
| ethylbenzene | $C_8H_{10}$ | 8.77 | 9.08 | 8.46 | 8.45 | 8.64 | 8.63 |

**Table S1:** Continued

| name | formula | Exp | $G_0W_0$ HF | BLYP | PBE | B3LYP | PBE0 |
|---|---|---|---|---|---|---|---|
| hexafluorobenzene | $C_6F_6$ | 10.20 | 10.59 | 9.35 | 9.33 | 9.69 | 9.70 |
| phenol | $C_6H_5OH$ | 8.75 | 8.99 | 8.23 | 8.24 | 8.44 | 8.45 |
| aniline | $C_6H_5NH_2$ | 8.05 | 8.31 | 7.52 | 7.53 | 7.74 | 7.76 |
| pyridine | $C_5H_5N$ | 9.51 | 9.87 | 8.96 | 9.01 | 9.35 | 9.46 |
| guanine | $C_5H_5N_5O$ | 8.24 | 8.40 | 7.54 | 7.54 | 7.78 | 7.80 |
| adenine | $C_5H_5N_5O$ | 8.48 | 8.66 | 7.82 | 7.83 | 8.06 | 8.08 |
| cytosine | $C_4H_5N_3O$ | 8.94 | 9.24 | 8.15 | 8.18 | 8.46 | 8.51 |
| thymine | $C_5H_6N_2O_2$ | 9.20 | 9.64 | 8.58 | 8.58 | 8.86 | 8.90 |
| uracil | $C_4H_4N_2O_2$ | 9.68 | 10.05 | 9.17 | 9.23 | 9.25 | 9.29 |
| urea | $CH_4N_2O$ | 10.15 | 10.65 | 9.23 | 9.29 | 9.64 | 9.73 |

**Table S2:** Ionization potentials of the GW100 set[S2] obtained from ev$GW_0$ and ev$GW$ with HF, BLYP, PBE, B3LYP and PBE0. The def2-TZVPP basis set was used. Systems containing Xe, Rb, I, Ag and Cu were excluded because of the convergence problem. All values in eV.

| | | | ev$GW_0$ | | | | | ev$GW$ | | | | |
|---|---|---|---|---|---|---|---|---|---|---|---|---|
| name | formula | Exp | HF | BLYP | PBE | B3LYP | PBE0 | HF | BLYP | PBE | B3LYP | PBE0 |
| helium | He | 24.59 | 24.60 | 24.20 | 24.25 | 24.32 | 24.36 | 24.58 | 24.63 | 24.67 | 24.62 | 24.64 |
| neon | Ne | 21.56 | 21.33 | 21.09 | 21.12 | 21.12 | 21.15 | 21.25 | 21.71 | 21.72 | 21.56 | 21.54 |
| argon | Ar | 15.76 | 15.71 | 15.27 | 15.25 | 15.33 | 15.33 | 15.68 | 15.58 | 15.55 | 15.55 | 15.52 |
| krypton | Kr | 14.00 | 13.94 | 13.55 | 13.52 | 13.59 | 13.58 | 13.92 | 13.81 | 13.77 | 13.77 | 13.74 |
| hydrogen | $H_2$ | 15.43 | 16.51 | 16.26 | 16.28 | 16.34 | 16.37 | 16.51 | 16.52 | 16.53 | 16.52 | 16.52 |
| lithium dimer | $Li_2$ | 4.73 | 5.34 | 5.20 | 5.22 | 5.23 | 5.26 | 5.34 | 5.32 | 5.33 | 5.29 | 5.31 |
| sodium dimer | $Na_2$ | 4.89 | 4.99 | 4.97 | 4.98 | 4.98 | 4.99 | 5.00 | 5.03 | 5.04 | 5.01 | 5.01 |
| sodium tetramer | $Na_4$ | 4.27 | 4.30 | 4.16 | 4.18 | 4.20 | 4.22 | 4.31 | 4.21 | 4.23 | 4.22 | 4.23 |
| sodium hexamer | $Na_6$ | 4.12 | 4.48 | 4.33 | 4.32 | 4.35 | 4.35 | 4.49 | 4.41 | 4.40 | 4.39 | 4.38 |
| potassium dimer | $K_2$ | 4.06 | 4.09 | 4.02 | 4.01 | 4.03 | 4.02 | 4.10 | 4.04 | 4.03 | 4.03 | 4.02 |
| nitrogen | $N_2$ | 15.58 | 17.12 | 15.25 | 15.28 | 15.45 | 15.53 | 17.10 | 15.71 | 15.73 | 15.78 | 15.82 |
| phosphorus dimer | $P_2$ | 10.62 | 10.55 | 10.13 | 10.12 | 10.21 | 10.22 | 10.55 | 10.32 | 10.31 | 10.33 | 10.32 |
| arsenic dimer | $As_2$ | 10.00 | 6.33 | 9.30 | 9.30 | 9.37 | 9.38 | 6.33 | 9.44 | 9.43 | 9.45 | 9.46 |
| fluorine | $F_2$ | 15.70 | 16.21 | 15.48 | 15.53 | 15.62 | 15.69 | 16.12 | 16.10 | 16.14 | 16.06 | 16.08 |
| chlorine | $Cl_2$ | 11.49 | 11.74 | 11.18 | 11.16 | 11.26 | 11.28 | 11.70 | 11.46 | 11.43 | 11.46 | 11.45 |

**Table S2:** Continued

| name | formula | Exp | ev$GW_0$ HF | ev$GW_0$ BLYP | ev$GW_0$ PBE | ev$GW_0$ B3LYP | ev$GW_0$ PBE0 | ev$GW$ HF | ev$GW$ BLYP | ev$GW$ PBE | ev$GW$ B3LYP | ev$GW$ PBE0 |
|---|---|---|---|---|---|---|---|---|---|---|---|---|
| bromine | $Br_2$ | 10.51 | | | 10.15 | | 10.25 | 10.66 | 10.43 | 10.40 | 10.41 | 10.40 |
| methane | $CH_4$ | 14.35 | 14.76 | 14.28 | 14.25 | 14.36 | 14.36 | 14.73 | 14.60 | 14.57 | 14.59 | 14.56 |
| ethane | $C_2H_6$ | 12.20 | 13.16 | 12.68 | 12.64 | 12.76 | 12.75 | 13.13 | 12.98 | 12.94 | 12.96 | 12.93 |
| propane | $C_3H_8$ | 11.51 | 12.61 | 12.11 | 12.06 | 12.19 | 12.17 | 12.57 | 12.41 | 12.36 | 12.40 | 12.35 |
| butane | $C_4H_{10}$ | 11.09 | 12.16 | 11.81 | 11.76 | 11.90 | 11.87 | 12.11 | 12.12 | 12.06 | 12.10 | 12.05 |
| ethylene | $C_2H_4$ | 10.68 | 10.77 | 10.43 | 10.40 | 10.48 | 10.48 | 10.76 | 10.63 | 10.59 | 10.61 | 10.58 |
| ethyn | $C_2H_2$ | 11.49 | 11.60 | 11.16 | 11.15 | 11.24 | 11.25 | 11.59 | 11.40 | 11.38 | 11.40 | 11.39 |
| tetracarbon | $C_4$ | 12.54 | 11.61 | 11.04 | 11.06 | 11.10 | 11.16 | 11.58 | 11.41 | 11.43 | 11.29 | 11.31 |
| cyclopropane | $C_3H_6$ | 10.54 | 11.28 | 10.74 | 10.70 | 10.82 | 10.81 | 11.24 | 11.02 | 10.97 | 11.00 | 10.97 |
| benzene | $C_6H_6$ | 9.23 | 9.52 | 9.07 | 9.03 | 9.14 | 9.13 | 9.49 | 9.29 | 9.24 | 9.28 | 9.24 |
| cyclooctatetraene | $C_8H_8$ | 8.43 | 8.68 | 8.13 | 8.09 | 8.23 | 8.21 | 8.65 | 8.33 | 8.28 | 8.35 | 8.32 |
| cyclopentadiene | $C_5H_6$ | 8.53 | 8.87 | 8.43 | 8.39 | 8.50 | 8.49 | 8.85 | 8.63 | 8.58 | 8.63 | 8.59 |
| vinyl fluoride | $C_2H_3F$ | 10.63 | 10.82 | 10.30 | 10.28 | 10.38 | 10.38 | 10.80 | 10.55 | 10.52 | 10.54 | 10.51 |
| vinyl chloride | $C_2H_3Cl$ | 10.20 | 10.36 | 9.82 | 9.80 | 9.92 | 9.92 | 10.34 | 10.06 | 10.02 | 10.07 | 10.04 |
| vinyl bromide | $C_2H_3Br$ | 9.90 | 9.45 | 8.98 | 8.94 | 9.05 | 9.04 | 9.43 | 9.18 | 9.14 | 9.18 | 9.15 |
| tetrafluoromethane | $CF_4$ | 16.20 | 16.75 | 15.82 | 15.85 | 16.02 | 16.09 | 16.60 | 16.47 | 16.50 | 16.46 | 16.47 |
| tetrachloromethane | $CCl_4$ | 11.69 | 11.96 | 11.15 | 11.13 | 11.31 | 11.33 | 11.88 | 11.53 | 11.50 | 11.56 | 11.54 |
| tetrabromomethane | $CBr_4$ | 10.54 | 10.71 | 9.95 | | 10.08 | 10.09 | 10.64 | 10.30 | 10.25 | 10.31 | 10.28 |
| silane | $SiH_4$ | 12.82 | 13.23 | 12.68 | 12.65 | 12.80 | 12.80 | 13.22 | 13.00 | 12.97 | 13.02 | 13.00 |
| germane | $GeH_4$ | 12.46 | 12.87 | 12.31 | 12.29 | 12.42 | 12.43 | 12.85 | 12.61 | 12.58 | 12.62 | 12.60 |
| disilane | $Si_2H_6$ | 10.53 | 11.09 | 10.50 | 10.42 | 10.60 | 10.56 | 11.07 | 10.74 | 10.65 | 10.76 | 10.69 |
| pentasilane | $Si_5H_{12}$ | 9.36 | 9.79 | 9.10 | 9.00 | 9.21 | 9.15 | 9.76 | 9.33 | 9.22 | 9.36 | 9.28 |
| lithium hydride | LiH | 7.90 | 8.16 | 7.63 | 7.70 | 7.83 | 7.91 | 8.16 | 8.18 | 8.22 | 8.16 | 8.19 |
| potassium hydride | KH | 8.00 | 6.29 | 5.69 | 5.73 | 5.88 | 5.95 | 6.26 | 6.34 | 6.36 | 6.29 | 6.30 |
| borane | $BH_3$ | 12.03 | 13.67 | 13.22 | 13.22 | 13.32 | 13.34 | 13.66 | 13.52 | 13.51 | 13.53 | 13.52 |
| diborane | $B_2H_6$ | 11.90 | 12.80 | 12.21 | 12.17 | 12.33 | 12.33 | 12.78 | 12.53 | 12.49 | 12.55 | 12.52 |
| ammonia | $NH_3$ | 10.82 | 11.16 | 10.66 | 10.68 | 10.73 | 10.77 | 11.13 | 11.04 | 11.04 | 10.99 | 11.00 |
| hydrazoic acid | $HN_3$ | 10.72 | 11.08 | 10.42 | 10.44 | 10.56 | 10.60 | 11.05 | 10.71 | 10.72 | 10.74 | 10.76 |
| phosphine | $PH_3$ | 10.59 | 10.80 | 10.42 | 10.37 | 10.48 | 10.46 | 10.79 | 10.61 | 10.56 | 10.61 | 10.57 |
| arsine | $AsH_3$ | 10.58 | 10.57 | 10.22 | 10.17 | 10.26 | 10.24 | 10.56 | 10.39 | 10.34 | 10.37 | 10.34 |
| hydrogen sulfide | $SH_2$ | 10.50 | 10.51 | 10.13 | 10.09 | 10.18 | 10.16 | 10.49 | 10.35 | 10.30 | 10.33 | 10.29 |
| hydrogen fluoride | FH | 16.12 | 16.14 | 15.81 | 15.86 | 15.86 | 15.90 | 16.07 | 16.38 | 16.40 | 16.25 | 16.25 |

**Table S2:** Continued

| name | formula | Exp | ev$GW_0$ | | | | | ev$GW$ | | | | |
|---|---|---|---|---|---|---|---|---|---|---|---|---|
| | | | HF | BLYP | PBE | B3LYP | PBE0 | HF | BLYP | PBE | B3LYP | PBE0 |
| hydrogen chloride | ClH | 12.79 | 12.77 | 12.37 | 12.33 | 12.42 | 12.42 | 12.75 | 12.64 | 12.61 | 12.61 | 12.58 |
| lithium fluoride | LiF | 11.30 | 11.23 | 10.90 | 10.94 | 11.00 | 11.04 | 11.12 | 11.70 | 11.72 | 11.50 | 11.47 |
| magnesium fluoride | $F_2Mg$ | 13.30 | 13.70 | 13.26 | 13.30 | 13.38 | 13.44 | 13.59 | 14.06 | 14.09 | 13.89 | 13.88 |
| titanium tetrafluoride | $TiF_4$ | | 15.92 | 14.64 | 14.67 | 14.94 | 15.04 | 15.65 | 15.56 | 15.59 | 15.54 | 15.56 |
| aluminum fluoride | $AlF_3$ | 15.45 | 15.51 | 14.89 | 14.93 | 15.03 | 15.10 | 15.39 | 15.59 | 15.63 | 15.49 | 15.51 |
| boron monofluoride | BF | 11.00 | 11.33 | 10.76 | 10.76 | 10.91 | 10.95 | 11.32 | 11.01 | 11.00 | 11.06 | 11.08 |
| sulfur tetrafluoride | $SF_4$ | 12.00 | 13.26 | 12.32 | 12.30 | 12.48 | 12.49 | 13.18 | 12.74 | 12.71 | 12.75 | 12.72 |
| potassium bromide | BrK | 8.82 | 8.16 | 7.79 | 7.77 | 7.84 | 7.84 | 8.13 | 8.19 | 8.14 | 8.08 | 8.04 |
| gallium monochloride | GaCl | 10.07 | 9.92 | 9.57 | 9.55 | 9.61 | 9.61 | 9.92 | 9.73 | 9.71 | 9.70 | 9.69 |
| sodium chloride | NaCl | 9.80 | 9.17 | 8.78 | 8.74 | 8.84 | 8.85 | 9.14 | 9.26 | 9.21 | 9.15 | 9.10 |
| magnesium chloride | $MgCl_2$ | 11.80 | 11.86 | 11.32 | 11.32 | 11.43 | 11.45 | 11.82 | 11.73 | 11.71 | 11.69 | 11.68 |
| boron nitride | BN | | 11.74 | 11.44 | | 11.54 | 11.59 | 11.71 | 11.83 | 11.86 | 11.79 | 11.81 |
| hydrogen cyanide | NCH | 13.61 | 13.87 | 13.37 | 13.38 | 13.48 | 13.51 | 13.85 | 13.70 | 13.69 | 13.69 | 13.69 |
| phosphorus mononitr | PN | 11.88 | 12.36 | 11.47 | 11.53 | 11.63 | 11.73 | 12.34 | 11.91 | 11.96 | 11.94 | 12.00 |
| hydrazine | $H_2NNH_2$ | 8.98 | 10.14 | 9.57 | 9.58 | 9.65 | 9.69 | 10.09 | 9.94 | 9.94 | 9.90 | 9.91 |
| formaldehyde | $H_2CO$ | 10.89 | 11.32 | 10.69 | 10.73 | 10.80 | 10.86 | 11.27 | 11.12 | 11.15 | 11.08 | 11.11 |
| methanol | $CH_4O$ | 10.96 | 11.52 | 10.89 | 10.93 | 10.98 | 11.03 | 11.46 | 11.35 | 11.36 | 11.28 | 11.29 |
| ethanol | $C_2H_6O$ | 10.64 | 11.24 | 10.52 | 10.54 | 10.62 | 10.67 | 11.17 | 11.00 | 11.00 | 10.93 | 10.93 |
| acetaldehyde | $C_2H_4O$ | 10.24 | 10.75 | 9.97 | 9.99 | 10.10 | 10.16 | 10.68 | 10.45 | 10.46 | 10.42 | 10.43 |
| ethoxy ethane | $C_4H_{10}O$ | 9.61 | 10.43 | 9.66 | 9.68 | 9.78 | 9.83 | 10.35 | 10.13 | 10.14 | 10.08 | 10.09 |
| formic acid | $CH_2O_2$ | 11.50 | 11.88 | | 11.18 | 11.29 | 11.36 | 11.79 | 11.66 | 11.68 | 11.63 | 11.65 |
| hydrogen peroxide | HOOH | 11.70 | 12.00 | 11.33 | 11.38 | 11.45 | 11.52 | 11.91 | 11.83 | 11.87 | 11.79 | 11.81 |
| water | $H_2O$ | 12.62 | 12.81 | 12.38 | 12.41 | 12.43 | 12.48 | 12.75 | 12.84 | 12.87 | 12.76 | 12.77 |
| carbon dioxide | $CO_2$ | 13.77 | 14.17 | 13.43 | 13.47 | 13.57 | 13.65 | 14.10 | 13.84 | 13.88 | 13.85 | 13.89 |
| carbon disulfide | $CS_2$ | 10.09 | 10.31 | 9.75 | 9.73 | 9.82 | 9.84 | 10.29 | 9.93 | 9.91 | 9.96 | 9.95 |
| carbon oxide sulfide | OCS | 11.19 | 11.53 | 10.91 | 10.90 | 11.02 | 11.04 | 11.50 | 11.15 | 11.14 | 11.18 | 11.18 |
| carbon oxide selenide | OCSe | 10.37 | 10.67 | 10.12 | 10.11 | 10.21 | 10.22 | | 10.32 | 10.30 | 10.34 | 10.33 |
| carbon monoxide | CO | 14.01 | 15.03 | 13.87 | 13.90 | 14.12 | 14.20 | 14.99 | 14.25 | 14.26 | 14.37 | 14.41 |
| ozone | $O_3$ | 12.73 | 13.53 | 12.38 | 12.40 | 12.61 | 12.70 | 13.47 | 12.91 | 12.93 | 12.99 | 13.03 |
| sulfur dioxide | $SO_2$ | 12.50 | 12.90 | 12.01 | 12.02 | 12.16 | 12.22 | 12.83 | 12.39 | 12.40 | 12.42 | 12.44 |
| beryllium monoxide | BeO | 10.10 | 9.73 | 9.84 | 9.88 | 9.78 | 9.81 | 9.65 | 10.45 | 10.48 | 10.18 | 10.15 |
| magnesium monoxide | MgO | 8.76 | 8.37 | 7.80 | 7.80 | 7.72 | 7.70 | 8.29 | 8.53 | 8.53 | 8.22 | 8.14 |

**Table S2:** Continued

| name | formula | Exp | ev$GW_0$ | | | | | ev$GW$ | | | | |
|---|---|---|---|---|---|---|---|---|---|---|---|---|
| | | | HF | BLYP | PBE | B3LYP | PBE0 | HF | BLYP | PBE | B3LYP | PBE0 |
| toluene | $C_7H_8$ | 8.82 | 9.15 | 8.70 | 8.66 | 8.77 | 8.76 | 9.12 | 8.92 | 8.87 | 8.91 | 8.87 |
| ethylbenzene | $C_8H_{10}$ | 8.77 | 9.12 | 8.65 | 8.61 | 8.72 | 8.70 | 9.09 | 8.87 | 8.82 | 8.86 | 8.82 |
| hexafluorobenzene | $C_6F_6$ | 10.20 | 10.61 | 9.60 | 9.56 | 9.80 | 9.79 | 10.55 | 9.89 | 9.84 | 9.97 | 9.94 |
| phenol | $C_6H_5OH$ | 8.75 | 9.02 | 8.46 | 8.44 | 8.53 | 8.53 | 8.98 | 8.72 | 8.70 | 8.69 | 8.66 |
| aniline | $C_6H_5NH_2$ | 8.05 | 8.34 | 7.75 | 7.73 | 7.83 | 7.84 | 8.30 | 8.02 | 8.00 | 7.99 | 7.98 |
| pyridine | $C_5H_5N$ | 9.51 | 9.91 | 9.41 | 9.43 | 9.59 | 9.66 | 9.89 | 9.86 | 9.88 | 9.88 | 9.91 |
| guanine | $C_5H_5N_5O$ | 8.24 | 8.43 | 7.72 | 7.70 | 7.85 | 7.86 | 8.38 | 7.96 | 7.93 | 8.00 | 7.98 |
| adenine | $C_5H_5N_5O$ | 8.48 | 8.70 | 8.02 | 8.00 | 8.14 | 8.14 | 8.65 | 8.28 | 8.25 | 8.29 | 8.27 |
| cytosine | $C_4H_5N_3O$ | 8.94 | 9.25 | 8.44 | 8.44 | 8.58 | 8.61 | 9.18 | 8.80 | 8.80 | 8.80 | 8.80 |
| thymine | $C_5H_6N_2O_2$ | 9.20 | 9.67 | 8.81 | 8.78 | 8.96 | 8.98 | 9.61 | 9.09 | 9.06 | 9.14 | 9.13 |
| uracil | $C_4H_4N_2O_2$ | 9.68 | 10.07 | 9.75 | 9.79 | 9.35 | 9.37 | 10.01 | 10.36 | 10.39 | 9.54 | 9.53 |
| urea | $CH_4N_2O$ | 10.15 | 10.63 | 9.75 | 9.78 | 9.88 | 9.95 | 10.54 | 10.31 | 10.33 | 10.24 | 10.26 |

**Table S3:** Ionization potentials of the GW100 set[S2] obtained from $G_{\mathrm{RS}}W_0$ and $G_{\mathrm{RS}}W_{\mathrm{RS}}$ with HF, BLYP, PBE, B3LYP and PBE0. The def2-TZVPP basis set was used. Systems containing Xe, Rb, I, Ag and Cu were excluded because of the convergence problem. All values in eV.

| name | formula | Exp | $G_{\mathrm{RS}}W_0$ | | | | | $G_{\mathrm{RS}}W_{\mathrm{RS}}$ | | | | |
|---|---|---|---|---|---|---|---|---|---|---|---|---|
| | | | HF | BLYP | PBE | B3LYP | PBE0 | HF | BLYP | PBE | B3LYP | PBE0 |
| helium | He | 24.59 | 24.60 | 24.29 | 24.34 | 24.37 | 24.41 | 24.60 | 24.67 | 24.71 | 24.66 | 24.67 |
| neon | Ne | 21.56 | 21.41 | 21.34 | 21.36 | 21.31 | 21.32 | 21.41 | 21.90 | 21.92 | 21.74 | 21.71 |
| argon | Ar | 15.76 | 15.73 | 15.37 | 15.35 | 15.40 | 15.39 | 15.73 | 15.65 | 15.62 | 15.61 | 15.58 |
| krypton | Kr | 14.00 | 13.96 | 13.65 | 13.62 | 13.66 | 13.64 | 13.96 | 13.88 | 13.84 | 13.83 | 13.79 |
| hydrogen | $H_2$ | 15.43 | 16.49 | 16.29 | 16.31 | 16.34 | 16.36 | 16.49 | 16.51 | 16.53 | 16.50 | 16.51 |
| lithium dimer | $Li_2$ | 4.73 | 5.29 | 5.15 | 5.17 | 5.17 | 5.20 | 5.29 | 5.29 | 5.30 | 5.27 | 5.28 |
| sodium dimer | $Na_2$ | 4.89 | 4.95 | 4.90 | 4.91 | 4.91 | 4.92 | 4.95 | 4.98 | 4.98 | 4.95 | 4.95 |
| sodium tetramer | $Na_4$ | 4.27 | 4.26 | 4.08 | 4.11 | 4.12 | 4.15 | 4.26 | 4.15 | 4.17 | 4.16 | 4.17 |
| sodium hexamer | $Na_6$ | 4.12 | 4.43 | 4.26 | 4.25 | 4.27 | 4.28 | 4.43 | 4.35 | 4.34 | 4.33 | 4.32 |
| potassium dimer | $K_2$ | 4.06 | 4.05 | 3.93 | 3.92 | 3.96 | 3.95 | 4.05 | 4.00 | 3.99 | 3.99 | 3.98 |
| nitrogen | $N_2$ | 15.58 | 17.10 | 15.42 | 15.44 | 15.56 | 15.62 | 17.10 | 15.81 | 15.83 | 15.87 | 15.90 |
| phosphorus dimer | $P_2$ | 10.62 | 10.52 | 10.12 | 10.11 | 10.18 | 10.20 | 10.52 | 10.30 | 10.28 | 10.30 | 10.30 |
| arsenic dimer | $As_2$ | 10.00 | 6.31 | 9.29 | 9.28 | 9.35 | 9.36 | 6.31 | 9.43 | 9.42 | 9.44 | 9.44 |

**Table S3:** Continued

| name | formula | Exp | $G_{RS}W_0$ | | | | | $G_{RS}W_{RS}$ | | | | |
|---|---|---|---|---|---|---|---|---|---|---|---|---|
| | | | HF | BLYP | PBE | B3LYP | PBE0 | HF | BLYP | PBE | B3LYP | PBE0 |
| fluorine | $F_2$ | 15.70 | 16.32 | 15.76 | 15.81 | 15.81 | 15.87 | 16.32 | 16.31 | 16.35 | 16.25 | 16.27 |
| chlorine | $Cl_2$ | 11.49 | 11.75 | 11.26 | 11.24 | 11.32 | 11.33 | 11.75 | 11.52 | 11.50 | 11.52 | 11.51 |
| bromine | $Br_2$ | 10.51 | 10.71 | 10.27 | 10.24 | 10.30 | 10.30 | 10.71 | 10.49 | 10.46 | 10.47 | 10.46 |
| methane | $CH_4$ | 14.35 | 14.75 | 14.35 | 14.32 | 14.40 | 14.39 | 14.75 | 14.64 | 14.60 | 14.61 | 14.58 |
| ethane | $C_2H_6$ | 12.20 | 13.16 | 12.74 | 12.70 | 12.79 | 12.77 | 13.16 | 13.01 | 12.97 | 13.00 | 12.96 |
| propane | $C_3H_8$ | 11.51 | 12.60 | 12.18 | 12.13 | 12.22 | 12.20 | 12.60 | 12.46 | 12.41 | 12.44 | 12.39 |
| butane | $C_4H_{10}$ | 11.09 | 12.15 | 11.87 | 11.82 | 11.92 | 11.90 | 12.15 | 12.17 | 12.11 | 12.15 | 12.09 |
| ethylene | $C_2H_4$ | 10.68 | 10.73 | 10.40 | 10.36 | 10.44 | 10.43 | 10.73 | 10.60 | 10.57 | 10.58 | 10.55 |
| ethyn | $C_2H_2$ | 11.49 | 11.56 | 11.14 | 11.14 | 11.21 | 11.22 | 11.56 | 11.38 | 11.37 | 11.37 | 11.37 |
| tetracarbon | $C_4$ | 12.54 | 11.59 | 11.09 | 11.11 | 11.12 | 11.16 | 11.59 | 11.44 | 11.45 | 11.30 | 11.32 |
| cyclopropane | $C_3H_6$ | 10.54 | 11.26 | 10.79 | 10.75 | 10.83 | 10.82 | 11.26 | 11.05 | 11.00 | 11.03 | 10.99 |
| benzene | $C_6H_6$ | 9.23 | 9.48 | 9.07 | 9.03 | 9.12 | 9.10 | 9.48 | 9.28 | 9.23 | 9.27 | 9.23 |
| cyclooctatetraene | $C_8H_8$ | 8.43 | 8.64 | 8.10 | 8.06 | 8.18 | 8.17 | 8.64 | 8.32 | 8.27 | 8.34 | 8.31 |
| cyclopentadiene | $C_5H_6$ | 8.53 | 8.82 | 8.40 | 8.36 | 8.46 | 8.44 | 8.82 | 8.61 | 8.56 | 8.60 | 8.57 |
| vinyl fluoride | $C_2H_3F$ | 10.63 | 10.80 | 10.33 | 10.30 | 10.38 | 10.37 | 10.80 | 10.58 | 10.55 | 10.55 | 10.53 |
| vinyl chloride | $C_2H_3Cl$ | 10.20 | 10.34 | 9.84 | 9.81 | 9.91 | 9.91 | 10.34 | 10.07 | 10.03 | 10.07 | 10.05 |
| vinyl bromide | $C_2H_3Br$ | 9.90 | 9.42 | 8.99 | 8.95 | 9.04 | 9.03 | 9.42 | 9.18 | 9.14 | 9.18 | 9.15 |
| tetrafluoromethane | $CF_4$ | 16.20 | 16.84 | 16.16 | 16.19 | 16.27 | 16.31 | 16.84 | 16.77 | 16.78 | 16.73 | 16.74 |
| tetrachloromethane | $CCl_4$ | 11.69 | 11.97 | 11.28 | 11.25 | 11.39 | 11.39 | 11.97 | 11.65 | 11.62 | 11.67 | 11.65 |
| tetrabromomethane | $CBr_4$ | 10.54 | 10.72 | 10.09 | 10.04 | 10.16 | 10.16 | 10.72 | 10.41 | 10.36 | 10.41 | 10.38 |
| silane | $SiH_4$ | 12.82 | 13.22 | 12.74 | 12.72 | 12.83 | 12.82 | 13.22 | 13.03 | 12.99 | 13.04 | 13.01 |
| germane | $GeH_4$ | 12.46 | 12.86 | 12.37 | 12.35 | 12.45 | 12.45 | 12.86 | 12.63 | 12.60 | 12.64 | 12.62 |
| disilane | $Si_2H_6$ | 10.53 | 11.07 | 10.53 | 10.45 | 10.60 | 10.55 | 11.07 | 10.75 | 10.66 | 10.76 | 10.70 |
| pentasilane | $Si_5H_{12}$ | 9.36 | 9.77 | 9.13 | 9.02 | 9.21 | 9.15 | 9.77 | 9.34 | 9.23 | 9.38 | 9.29 |
| lithium hydride | LiH | 7.90 | 8.15 | 7.89 | 7.94 | 7.93 | 7.99 | 8.15 | 8.21 | 8.25 | 8.18 | 8.21 |
| potassium hydride | KH | 8.00 | 6.29 | 6.09 | 6.12 | 6.08 | 6.11 | 6.29 | 6.41 | 6.44 | 6.35 | 6.36 |
| borane | $BH_3$ | 12.03 | 13.65 | 13.28 | 13.27 | 13.34 | 13.35 | 13.65 | 13.53 | 13.52 | 13.53 | 13.52 |
| diborane | $B_2H_6$ | 11.90 | 12.79 | 12.28 | 12.24 | 12.36 | 12.35 | 12.79 | 12.56 | 12.51 | 12.57 | 12.54 |
| ammonia | $NH_3$ | 10.82 | 11.17 | 10.78 | 10.79 | 10.80 | 10.83 | 11.17 | 11.10 | 11.10 | 11.05 | 11.05 |
| hydrazoic acid | $HN_3$ | 10.72 | 11.06 | 10.47 | 10.49 | 10.57 | 10.61 | 11.06 | 10.74 | 10.75 | 10.77 | 10.79 |
| phosphine | $PH_3$ | 10.59 | 10.77 | 10.42 | 10.38 | 10.46 | 10.44 | 10.77 | 10.60 | 10.55 | 10.60 | 10.55 |
| arsine | $AsH_3$ | 10.58 | 10.56 | 10.23 | 10.19 | 10.26 | 10.23 | 10.56 | 10.38 | 10.34 | 10.37 | 10.33 |

**Table S3:** Continued

| name | formula | Exp | $G_{\rm RS}W_0$ HF | BLYP | PBE | B3LYP | PBE0 | $G_{\rm RS}W_{\rm RS}$ HF | BLYP | PBE | B3LYP | PBE0 |
|---|---|---|---|---|---|---|---|---|---|---|---|---|
| hydrogen sulfide | $SH_2$ | 10.50 | 10.49 | 10.16 | 10.12 | 10.19 | 10.17 | 10.49 | 10.37 | 10.32 | 10.34 | 10.30 |
| hydrogen fluoride | FH | 16.12 | 16.21 | 16.06 | 16.09 | 16.03 | 16.06 | 16.21 | 16.55 | 16.58 | 16.41 | 16.41 |
| hydrogen chloride | ClH | 12.79 | 12.78 | 12.43 | 12.41 | 12.46 | 12.45 | 12.78 | 12.68 | 12.65 | 12.65 | 12.61 |
| lithium fluoride | LiF | 11.30 | 11.34 | 11.47 | 11.49 | 11.36 | 11.36 | 11.34 | 12.03 | 12.04 | 11.80 | 11.76 |
| magnesium fluoride | $F_2Mg$ | 13.30 | 13.82 | 13.82 | 13.85 | 13.74 | 13.75 | 13.82 | 14.40 | 14.43 | 14.20 | 14.17 |
| titanium tetrafluoride | $TiF_4$ | | 16.06 | 15.28 | 15.31 | 15.38 | 15.44 | 16.06 | 16.00 | 16.03 | 15.96 | 15.98 |
| aluminum fluoride | $AlF_3$ | 15.45 | 15.61 | 15.32 | 15.36 | 15.32 | 15.36 | 15.61 | 15.91 | 15.94 | 15.78 | 15.78 |
| boron monofluoride | BF | 11.00 | 11.30 | 10.77 | 10.77 | 10.89 | 10.93 | 11.30 | 11.00 | 10.99 | 11.05 | 11.06 |
| sulfur tetrafluoride | $SF_4$ | 12.00 | 13.30 | 12.51 | 12.49 | 12.61 | 12.61 | 13.30 | 12.90 | 12.87 | 12.90 | 12.87 |
| potassium bromide | BrK | 8.82 | 8.18 | 7.99 | 7.95 | 7.95 | 7.93 | 8.19 | 8.28 | 8.23 | 8.16 | 8.12 |
| gallium monochloride | GaCl | 10.07 | 9.91 | 9.61 | 9.59 | 9.62 | 9.62 | 9.91 | 9.75 | 9.72 | 9.71 | 9.70 |
| sodium chloride | NaCl | 9.80 | 9.20 | 9.04 | 9.00 | 8.99 | 8.97 | 9.20 | 9.37 | 9.33 | 9.24 | 9.19 |
| magnesium chloride | $MgCl_2$ | 11.80 | 11.88 | 11.49 | 11.48 | 11.53 | 11.54 | 11.88 | 11.83 | 11.81 | 11.78 | 11.76 |
| boron nitride | BN | | 11.71 | 11.50 | 11.53 | 11.55 | 11.59 | 11.71 | 11.84 | 11.87 | 11.79 | 11.81 |
| hydrogen cyanide | NCH | 13.61 | 13.85 | 13.40 | 13.40 | 13.47 | 13.50 | 13.85 | 13.71 | 13.70 | 13.69 | 13.69 |
| phosphorus mononitr | PN | 11.88 | 12.34 | 11.60 | 11.65 | 11.70 | 11.79 | 12.34 | 11.97 | 12.01 | 11.99 | 12.05 |
| hydrazine | $H_2NNH_2$ | 8.98 | 10.14 | 9.67 | 9.68 | 9.71 | 9.74 | 10.14 | 10.01 | 10.01 | 9.97 | 9.97 |
| formaldehyde | $H_2CO$ | 10.89 | 11.34 | 10.86 | 10.89 | 10.90 | 10.95 | 11.34 | 11.23 | 11.25 | 11.18 | 11.20 |
| methanol | $CH_4O$ | 10.96 | 11.54 | 11.06 | 11.09 | 11.08 | 11.12 | 11.54 | 11.48 | 11.49 | 11.39 | 11.40 |
| ethanol | $C_2H_6O$ | 10.64 | 11.26 | 10.71 | 10.72 | 10.73 | 10.77 | 11.26 | 11.14 | 11.14 | 11.06 | 11.06 |
| acetaldehyde | $C_2H_4O$ | 10.24 | 10.78 | 10.18 | 10.19 | 10.23 | 10.27 | 10.78 | 10.59 | 10.60 | 10.55 | 10.55 |
| ethoxy ethane | $C_4H_{10}O$ | 9.61 | 10.46 | 9.87 | 9.88 | 9.91 | 9.94 | 10.46 | 10.30 | 10.30 | 10.23 | 10.24 |
| formic acid | $CH_2O_2$ | 11.50 | 11.92 | 11.38 | 11.41 | 11.45 | 11.49 | 11.92 | 11.82 | 11.84 | 11.78 | 11.80 |
| hydrogen peroxide | HOOH | 11.70 | 12.04 | 11.55 | 11.59 | 11.59 | 11.65 | 12.04 | 11.99 | 12.02 | 11.93 | 11.96 |
| water | $H_2O$ | 12.62 | 12.85 | 12.56 | 12.59 | 12.56 | 12.59 | 12.85 | 12.97 | 12.99 | 12.88 | 12.88 |
| carbon dioxide | $CO_2$ | 13.77 | 14.20 | 13.56 | 13.63 | 13.66 | 13.73 | 14.20 | 13.95 | 13.99 | 13.96 | 13.99 |
| carbon disulfide | $CS_2$ | 10.09 | 10.29 | 9.75 | 9.74 | 9.83 | 9.84 | 10.29 | 9.93 | 9.91 | 9.96 | 9.96 |
| carbon oxide sulfide | OCS | 11.19 | 11.52 | 10.96 | 10.95 | 11.05 | 11.06 | 11.52 | 11.18 | 11.17 | 11.21 | 11.21 |
| carbon oxide selenide | OCSe | 10.37 | 10.66 | 10.16 | 10.14 | 10.23 | 10.24 | 10.66 | 10.35 | 10.33 | 10.37 | 10.36 |
| carbon monoxide | CO | 14.01 | 15.04 | 14.00 | 14.01 | 14.19 | 14.25 | 15.04 | 14.32 | 14.33 | 14.44 | 14.47 |
| ozone | $O_3$ | 12.73 | 13.53 | 12.63 | 12.65 | 12.78 | 12.84 | 13.53 | 13.07 | 13.09 | 13.15 | 13.18 |
| sulfur dioxide | $SO_2$ | 12.50 | 12.94 | 12.17 | 12.18 | 12.28 | 12.32 | 12.94 | 12.51 | 12.51 | 12.54 | 12.55 |

**Table S3:** Continued

| name | formula | Exp | $G_{RS}W_0$ | | | | | $G_{RS}W_{RS}$ | | | | |
|---|---|---|---|---|---|---|---|---|---|---|---|---|
| | | | HF | BLYP | PBE | B3LYP | PBE0 | HF | BLYP | PBE | B3LYP | PBE0 |
| beryllium monoxide | BeO | 10.10 | 9.78 | 10.19 | 10.22 | 9.99 | 9.99 | 9.78 | 10.59 | 10.62 | 10.31 | 10.28 |
| magnesium monoxide | MgO | 8.76 | 8.40 | 8.35 | 8.35 | 8.07 | 8.03 | 8.40 | 8.78 | 8.78 | 8.47 | 8.40 |
| toluene | $C_7H_8$ | 8.82 | 9.11 | 8.70 | 8.66 | 8.74 | 8.73 | 9.11 | 8.91 | 8.87 | 8.90 | 8.86 |
| ethylbenzene | $C_8H_{10}$ | 8.77 | 9.08 | 8.65 | 8.61 | 8.70 | 8.68 | 9.08 | 8.87 | 8.82 | 8.86 | 8.82 |
| hexafluorobenzene | $C_6F_6$ | 10.20 | 10.59 | 9.70 | 9.65 | 9.85 | 9.83 | 10.59 | 9.98 | 9.93 | 10.05 | 10.01 |
| phenol | $C_6H_5OH$ | 8.75 | 8.99 | 8.50 | 8.49 | 8.54 | 8.53 | 8.99 | 8.75 | 8.74 | 8.71 | 8.69 |
| aniline | $C_6H_5NH_2$ | 8.05 | 8.31 | 7.79 | 7.77 | 7.84 | 7.84 | 8.31 | 8.05 | 8.03 | 8.02 | 8.00 |
| pyridine | $C_5H_5N$ | 9.51 | 9.87 | 9.47 | 9.48 | 9.59 | 9.65 | 9.87 | 9.93 | 9.94 | 9.94 | 9.97 |
| guanine | $C_5H_5N_5O$ | 8.24 | 8.40 | 7.79 | 7.76 | 7.87 | 7.87 | 8.40 | 8.01 | 7.98 | 8.04 | 8.01 |
| adenine | $C_5H_5N_5O$ | 8.48 | 8.66 | 8.08 | 8.06 | 8.16 | 8.16 | 8.66 | 8.32 | 8.30 | 8.33 | 8.31 |
| cytosine | $C_4H_5N_3O$ | 8.94 | 9.24 | 8.56 | 8.56 | 8.64 | 8.67 | 9.24 | 8.88 | 8.88 | 8.88 | 8.88 |
| thymine | $C_5H_6N_2O_2$ | 9.20 | 9.64 | 8.89 | 8.87 | 8.99 | 9.00 | 9.64 | 9.16 | 9.13 | 9.19 | 9.18 |
| uracil | $C_4H_4N_2O_2$ | 9.68 | 10.05 | 9.88 | 9.90 | 9.39 | 9.41 | 10.05 | 10.50 | 10.52 | 9.60 | 9.59 |
| urea | $CH_4N_2O$ | 10.15 | 10.65 | 10.00 | 10.02 | 10.04 | 10.08 | 10.65 | 10.48 | 10.50 | 10.40 | 10.41 |

**Table S4:** Ionization potentials of the GW100 set[S2] obtained from $G_{RSc}W_0$ and $G_{RSc}W_{RSc}$ with HF, BLYP, PBE, B3LYP and PBE0. The def2-TZVPP basis set was used. Systems containing Xe, Rb, I, Ag and Cu were excluded because of the convergence problem. All values in eV.

| name | formula | Exp | $G_{RSc}W_0$ | | | | | $G_{RSc}W_{RSc}$ | | | | |
|---|---|---|---|---|---|---|---|---|---|---|---|---|
| | | | HF | BLYP | PBE | B3LYP | PBE0 | HF | BLYP | PBE | B3LYP | PBE0 |
| helium | He | 24.59 | 24.59 | 24.24 | 24.29 | 24.35 | 24.39 | 24.58 | 24.65 | 24.69 | 24.64 | 24.66 |
| neon | Ne | 21.56 | 21.34 | 21.20 | 21.23 | 21.20 | 21.22 | 21.27 | 21.77 | 21.78 | 21.62 | 21.59 |
| argon | Ar | 15.76 | 15.71 | 15.35 | 15.32 | 15.34 | 15.33 | 15.69 | 15.63 | 15.59 | 15.54 | 15.51 |
| krypton | Kr | 14.00 | | 13.62 | 13.58 | 13.65 | 13.64 | 13.92 | 13.85 | 13.81 | 13.81 | 13.78 |
| hydrogen | $H_2$ | 15.43 | 16.51 | 16.29 | 16.32 | 16.36 | 16.37 | 16.51 | 16.54 | 16.56 | 16.54 | 16.52 |
| lithium dimer | $Li_2$ | 4.73 | 5.34 | 5.22 | 5.23 | 5.24 | 5.26 | 5.37 | 5.34 | 5.35 | 5.31 | 5.32 |
| sodium dimer | $Na_2$ | 4.89 | 4.99 | 4.98 | 4.98 | 4.98 | 4.98 | 5.00 | 5.03 | 5.04 | 5.00 | 5.00 |
| sodium tetramer | $Na_4$ | 4.27 | 4.30 | 4.18 | 4.19 | 4.19 | 4.21 | 4.31 | 4.22 | 4.23 | 4.21 | 4.23 |
| sodium hexamer | $Na_6$ | 4.12 | 4.47 | 4.35 | 4.34 | 4.35 | 4.35 | 4.48 | 4.41 | 4.40 | 4.39 | 4.38 |
| potassium dimer | $K_2$ | 4.06 | 4.09 | 4.02 | 4.00 | 4.02 | 4.01 | 4.10 | 4.05 | 4.04 | 4.04 | 4.02 |
| nitrogen | $N_2$ | 15.58 | 17.12 | 15.35 | 15.38 | 15.51 | 15.59 | 17.10 | 15.76 | 15.78 | 15.81 | 15.85 |

**Table S4:** Continued

| name | formula | Exp | $G_{\mathrm{RSc}}W_0$ | | | | | $G_{\mathrm{RSc}}W_{\mathrm{RSc}}$ | | | | |
|---|---|---|---|---|---|---|---|---|---|---|---|---|
| | | | HF | BLYP | PBE | B3LYP | PBE0 | HF | BLYP | PBE | B3LYP | PBE0 |
| phosphorus dimer | $P_2$ | 10.62 | 10.55 | 10.19 | 10.18 | 10.25 | 10.25 | 10.54 | 10.34 | 10.33 | 10.35 | 10.34 |
| arsenic dimer | $As_2$ | 10.00 | 6.34 | 9.35 | 9.34 | | 9.41 | 6.33 | 9.46 | 9.45 | 9.46 | |
| fluorine | $F_2$ | 15.70 | 16.2 | 15.58 | 15.63 | 15.65 | 15.72 | 16.13 | 16.15 | 16.19 | 16.08 | 16.10 |
| chlorine | $Cl_2$ | 11.49 | 11.73 | 11.25 | 11.23 | 11.31 | 11.32 | 11.70 | 11.50 | 11.48 | 11.49 | 11.49 |
| bromine | $Br_2$ | 10.51 | 10.69 | | | | 10.28 | 10.66 | 10.47 | 10.44 | 10.45 | 10.43 |
| methane | $CH_4$ | 14.35 | 14.75 | 14.35 | 14.32 | 14.41 | 14.41 | 14.74 | 14.64 | 14.60 | 14.62 | 14.58 |
| ethane | $C_2H_6$ | 12.20 | 13.16 | 12.75 | 12.71 | 12.8 | 12.79 | 13.14 | 13.01 | 12.96 | 12.99 | 12.95 |
| propane | $C_3H_8$ | 11.51 | 12.61 | 12.18 | 12.13 | 12.24 | 12.21 | 12.58 | 12.45 | 12.39 | 12.43 | 12.38 |
| butane | $C_4H_{10}$ | 11.09 | 12.15 | 11.87 | 11.82 | 11.93 | 11.91 | 12.12 | 12.15 | 12.09 | 12.12 | 12.07 |
| ethylene | $C_2H_4$ | 10.68 | 10.77 | 10.47 | 10.44 | 10.51 | 10.49 | 10.76 | 10.66 | 10.61 | 10.63 | 10.60 |
| ethyn | $C_2H_2$ | 11.49 | 11.59 | 11.21 | 11.20 | 11.26 | 11.28 | 11.59 | 11.43 | 11.41 | 11.42 | 11.41 |
| tetracarbon | $C_4$ | 12.54 | 11.6 | 11.1 | 11.12 | 11.16 | 11.20 | 11.58 | 11.42 | 11.43 | 11.32 | 11.34 |
| cyclopropane | $C_3H_6$ | 10.54 | 11.27 | 10.82 | 10.78 | 10.87 | 10.85 | 11.24 | 11.06 | 11.01 | 11.04 | 10.99 |
| benzene | $C_6H_6$ | 9.23 | 9.51 | 9.15 | 9.11 | 9.19 | 9.17 | 9.50 | 9.33 | 9.28 | 9.30 | 9.27 |
| cyclooctatetraene | $C_8H_8$ | 8.43 | 8.67 | 8.19 | 8.15 | 8.26 | 8.24 | 8.65 | 8.37 | 8.32 | 8.38 | 8.34 |
| cyclopentadiene | $C_5H_6$ | 8.53 | 8.86 | 8.49 | 8.44 | 8.54 | 8.52 | 8.85 | 8.66 | 8.61 | 8.65 | 8.62 |
| vinyl fluoride | $C_2H_3F$ | 10.63 | 10.82 | 10.36 | 10.33 | 10.41 | 10.4 | 10.80 | 10.58 | 10.55 | 10.56 | 10.53 |
| vinyl chloride | $C_2H_3Cl$ | 10.20 | 10.36 | 9.89 | 9.86 | 9.95 | 9.95 | 10.34 | 10.09 | 10.05 | 10.09 | 10.07 |
| vinyl bromide | $C_2H_3Br$ | 9.90 | 9.45 | 9.03 | 9.00 | 9.08 | 9.07 | 9.43 | 9.20 | 9.16 | 9.20 | 9.17 |
| tetrafluoromethane | $CF_4$ | 16.20 | 16.74 | 15.99 | 16.02 | 16.13 | 16.19 | 16.63 | 16.55 | 16.57 | 16.53 | 16.53 |
| tetrachloromethane | $CCl_4$ | 11.69 | 11.95 | 11.25 | 11.23 | 11.37 | 11.38 | 11.89 | 11.60 | 11.56 | 11.61 | 11.59 |
| tetrabromomethane | $CBr_4$ | 10.54 | 10.71 | 10.06 | 10.01 | 10.15 | 10.14 | 10.65 | 10.35 | 10.30 | | 10.32 |
| silane | $SiH_4$ | 12.82 | 13.23 | 12.74 | 12.72 | 12.84 | 12.84 | 13.21 | 13.03 | 13.00 | 13.04 | 13.02 |
| germane | $GeH_4$ | 12.46 | 12.87 | 12.38 | 12.35 | | 12.46 | 12.85 | 12.63 | 12.60 | 12.64 | 12.62 |
| disilane | $Si_2H_6$ | 10.53 | 11.08 | 10.56 | 10.48 | 10.63 | 10.59 | 11.07 | 10.77 | 10.68 | 10.78 | 10.71 |
| pentasilane | $Si_5H_{12}$ | 9.36 | 9.78 | 9.17 | 9.07 | 9.25 | 9.19 | 9.76 | 9.36 | 9.25 | 9.39 | 9.30 |
| lithium hydride | LiH | 7.90 | 8.15 | 7.81 | 7.86 | 7.91 | 7.98 | 8.15 | 8.21 | 8.25 | 8.19 | 8.22 |
| potassium hydride | KH | 8.00 | 6.29 | 5.98 | 6.01 | 6.02 | 6.07 | 6.26 | 6.39 | 6.41 | 6.32 | 6.34 |
| borane | $BH_3$ | 12.03 | 13.66 | 13.28 | 13.28 | 13.36 | 13.37 | 13.65 | 13.55 | 13.53 | 13.54 | 13.53 |
| diborane | $B_2H_6$ | 11.90 | 12.79 | 12.28 | 12.24 | 12.37 | 12.36 | 12.78 | 12.56 | 12.51 | 12.57 | 12.54 |
| ammonia | $NH_3$ | 10.82 | 11.15 | 10.74 | 10.75 | 10.78 | 10.82 | 11.13 | 11.07 | 11.07 | 11.02 | 11.02 |
| hydrazoic acid | $HN_3$ | 10.72 | 11.08 | 10.52 | 10.53 | 10.62 | 10.65 | 11.05 | 10.76 | 10.77 | 10.78 | 10.80 |

**Table S4:** Continued

| | | | $G_{RSc}W_0$ | | | | | $G_{RSc}W_{RSc}$ | | | | |
|---|---|---|---|---|---|---|---|---|---|---|---|---|
| name | formula | Exp | HF | BLYP | PBE | B3LYP | PBE0 | HF | BLYP | PBE | B3LYP | PBE0 |
| phosphine | $PH_3$ | 10.59 | 10.79 | 10.46 | 10.42 | 10.5 | 10.48 | 10.79 | 10.63 | 10.59 | 10.63 | 10.59 |
| arsine | $AsH_3$ | 10.58 | 10.57 | 10.26 | 10.21 | 10.29 | 10.26 | 10.56 | 10.41 | 10.36 | 10.39 | 10.35 |
| hydrogen sulfide | $SH_2$ | 10.50 | 10.5 | 10.18 | 10.15 | 10.21 | 10.19 | 10.49 | 10.39 | 10.34 | 10.36 | 10.31 |
| hydrogen fluoride | FH | 16.12 | 16.14 | 15.94 | 15.98 | 15.93 | 15.98 | 16.08 | 16.44 | 16.46 | 16.29 | 16.29 |
| hydrogen chloride | ClH | 12.79 | 12.77 | 12.44 | 12.41 | 12.44 | 12.43 | 12.75 | 12.68 | 12.65 | 12.62 | 12.59 |
| lithium fluoride | LiF | 11.30 | 11.23 | 11.19 | 11.22 | 11.16 | 11.18 | 11.16 | 11.84 | 11.86 | 11.60 | 11.58 |
| magnesium fluoride | $F_2Mg$ | 13.30 | 13.70 | 13.54 | 13.57 | 13.54 | 13.57 | 13.61 | 14.18 | 14.21 | 13.99 | 13.97 |
| titanium tetrafluoride | $TiF_4$ | | 15.92 | 14.98 | 15.01 | 15.15 | 15.23 | 15.70 | 15.67 | 15.70 | 15.64 | 15.66 |
| aluminum fluoride | $AlF_3$ | 15.45 | 15.51 | 15.1 | 15.14 | 15.17 | 15.22 | 15.41 | 15.70 | 15.74 | 15.58 | 15.59 |
| boron monofluoride | BF | 11.00 | 11.33 | 10.82 | 10.82 | 10.94 | 10.98 | 11.32 | 11.04 | 11.03 | 11.08 | 11.10 |
| sulfur tetrafluoride | $SF_4$ | 12.00 | 13.26 | 12.44 | 12.41 | 12.56 | 12.56 | 13.20 | 12.79 | 12.76 | 12.80 | 12.77 |
| potassium bromide | BrK | 8.82 | 8.16 | 7.91 | 7.89 | 7.92 | 7.91 | 8.14 | 8.24 | 8.20 | 8.13 | 8.09 |
| gallium monochloride | GaCl | 10.07 | 9.92 | 9.62 | 9.61 | | 9.64 | 9.92 | 9.76 | 9.73 | 9.72 | 9.71 |
| sodium chloride | NaCl | 9.80 | 9.17 | 8.94 | 8.93 | 8.94 | 8.92 | 9.14 | 9.33 | 9.29 | 9.20 | 9.13 |
| magnesium chloride | $MgCl_2$ | 11.80 | 11.85 | 11.42 | 11.43 | 11.5 | 11.51 | 11.82 | 11.77 | 11.77 | 11.73 | 11.72 |
| boron nitride | BN | | 11.73 | 11.54 | 11.57 | 11.59 | 11.64 | 11.71 | 11.88 | 11.90 | 11.82 | 11.85 |
| hydrogen cyanide | NCH | 13.61 | 13.87 | 13.45 | 13.46 | 13.52 | 13.54 | 13.85 | 13.73 | 13.73 | 13.72 | 13.71 |
| phosphorus mononitr | PN | 11.88 | 12.36 | 11.51 | 11.57 | 11.64 | 11.74 | 12.33 | 11.91 | 11.96 | 11.92 | 11.98 |
| hydrazine | $H_2NNH_2$ | 8.98 | 10.13 | 9.65 | 9.66 | 9.70 | 9.73 | 10.09 | 9.98 | 9.98 | 9.93 | 9.93 |
| formaldehyde | $H_2CO$ | 10.89 | 11.31 | 10.80 | 10.83 | 10.86 | 10.91 | 11.27 | 11.17 | 11.19 | 11.12 | 11.14 |
| methanol | $CH_4O$ | 10.96 | 11.51 | 10.99 | 11.02 | 11.04 | 11.09 | 11.46 | 11.39 | 11.41 | 11.31 | 11.33 |
| ethanol | $C_2H_6O$ | 10.64 | 11.23 | 10.61 | 10.63 | 10.68 | 10.72 | 11.18 | 11.04 | 11.04 | 10.97 | 10.97 |
| acetaldehyde | $C_2H_4O$ | 10.24 | 10.74 | 10.08 | 10.10 | 10.17 | 10.22 | 10.69 | 10.50 | 10.51 | 10.46 | 10.47 |
| ethoxy ethane | $C_4H_{10}O$ | 9.61 | 10.41 | 9.77 | 9.79 | 9.85 | 9.89 | 10.36 | 10.18 | 10.19 | 10.13 | 10.13 |
| formic acid | $CH_2O_2$ | 11.50 | 11.87 | 11.28 | 11.32 | 11.38 | 11.44 | 11.80 | 11.72 | 11.74 | 11.68 | 11.70 |
| hydrogen peroxide | HOOH | 11.70 | 11.98 | 11.45 | 11.5 | 11.52 | 11.59 | 11.92 | 11.88 | 11.92 | 11.83 | 11.85 |
| water | $H_2O$ | 12.62 | 12.81 | 12.48 | 12.51 | 12.5 | 12.54 | 12.76 | 12.90 | 12.92 | 12.80 | 12.81 |
| carbon dioxide | $CO_2$ | 13.77 | 14.16 | 13.54 | 13.60 | 13.65 | 13.72 | 14.11 | 13.90 | 13.94 | 13.91 | 13.95 |
| carbon disulfide | $CS_2$ | 10.09 | 10.31 | 9.80 | 9.78 | 9.87 | 9.88 | 10.29 | 9.96 | 9.94 | 9.99 | 9.98 |
| carbon oxide sulfide | OCS | 11.19 | 11.52 | 10.98 | 10.98 | 11.07 | 11.09 | 11.49 | 11.19 | 11.17 | 11.21 | 11.21 |
| carbon oxide selenide | OCSe | 10.37 | 10.67 | 10.19 | 10.17 | 10.26 | 10.25 | 10.65 | 10.36 | | 10.38 | 10.36 |
| carbon monoxide | CO | 14.01 | 15.03 | 13.98 | 14 | 14.18 | 14.25 | 14.99 | 14.31 | 14.31 | 14.42 | 14.45 |

**Table S4:** Continued

| name | formula | Exp | $G_{RSc}W_0$ | | | | | $G_{RSc}W_{RSc}$ | | | | |
|---|---|---|---|---|---|---|---|---|---|---|---|---|
| | | | HF | BLYP | PBE | B3LYP | PBE0 | HF | BLYP | PBE | B3LYP | PBE0 |
| ozone | $O_3$ | 12.73 | 13.54 | 12.45 | 12.48 | 12.63 | 12.71 | 13.49 | 12.94 | 12.96 | 13.00 | 13.04 |
| sulfur dioxide | $SO_2$ | 12.50 | 12.9 | 12.1 | 12.11 | 12.22 | 12.27 | 12.84 | 12.44 | 12.44 | 12.46 | 12.48 |
| beryllium monoxide | BeO | 10.10 | 9.72 | 10.06 | 10.1 | 9.91 | 9.93 | 9.66 | 10.51 | 10.54 | 10.23 | 10.20 |
| magnesium monoxide | MgO | 8.76 | 8.34 | 7.90 | 7.92 | 7.72 | 7.71 | 8.28 | 8.52 | 8.54 | 8.19 | 8.15 |
| toluene | $C_7H_8$ | 8.82 | 9.15 | 8.78 | 8.73 | 8.81 | 8.79 | 9.13 | 8.95 | 8.91 | 8.93 | 8.89 |
| ethylbenzene | $C_8H_{10}$ | 8.77 | 9.11 | 8.73 | 8.68 | 8.77 | 8.74 | 9.09 | 8.91 | 8.86 | 8.89 | 8.85 |
| hexafluorobenzene | $C_6F_6$ | 10.20 | 10.6 | 9.70 | 9.65 | 9.86 | 9.84 | 10.56 | 9.94 | 9.89 | 10.01 | 9.97 |
| phenol | $C_6H_5OH$ | 8.75 | 9.01 | 8.54 | 8.52 | 8.57 | 8.57 | 8.98 | 8.75 | 8.73 | 8.71 | 8.69 |
| aniline | $C_6H_5NH_2$ | 8.05 | 8.33 | 7.84 | 7.82 | 7.88 | 7.88 | 8.30 | 8.05 | 8.03 | 8.02 | 8.00 |
| pyridine | $C_5H_5N$ | 9.51 | 9.91 | 9.33 | 9.35 | 9.48 | 9.55 | 9.89 | 9.78 | 9.79 | 9.79 | 9.82 |
| guanine | $C_5H_5N_5O$ | 8.24 | 8.42 | 7.85 | 7.82 | 7.92 | 7.92 | 8.39 | 8.03 | 8.00 | 8.04 | 8.02 |
| adenine | $C_5H_5N_5O$ | 8.48 | 8.69 | 8.15 | 8.12 | 8.21 | 8.21 | 8.66 | 8.34 | 8.31 | 8.34 | 8.32 |
| cytosine | $C_4H_5N_3O$ | 8.94 | 9.25 | 8.58 | 8.58 | 8.67 | 8.69 | 9.20 | 8.86 | 8.85 | 8.85 | 8.84 |
| thymine | $C_5H_6N_2O_2$ | 9.20 | 9.66 | 8.94 | 8.91 | 9.03 | 9.04 | 9.62 | 9.16 | 9.13 | 9.18 | 9.17 |
| uracil | $C_4H_4N_2O_2$ | 9.68 | 10.06 | 9.59 | 9.61 | 9.43 | 9.44 | 10.02 | 10.23 | 10.25 | 9.58 | 9.58 |
| urea | $CH_4N_2O$ | 10.15 | 10.62 | 9.86 | 9.89 | 9.96 | 10.01 | 10.55 | 10.33 | 10.35 | 10.27 | 10.28 |

# 3 Core-Level Binding Energies of the CORE65 Set obtained from Different *GW* Methods

**Table S5:** Core-level of the CORE65 set[S3] obtained from $G_0W_0$ with HF, BLYP, PBE, B3LYP and PBE0. The cc-pVTZ basis set was used. All values in eV.

| formula | core level | Ref | $G_0W_0$ | | | | |
|---|---|---|---|---|---|---|---|
| | | | HF | BLYP | PBE | B3LYP | PBE0 |
| $CH_4$ | C1s | 290.84 | 295.48 | | | 285.91 | 286.90 |
| $C_2H_6$ | C1s | 290.71 | 295.49 | | | 285.85 | 286.89 |
| $C_2H_4$ | C1s | 290.82 | 295.90 | | | 285.25 | 286.34 |
| $C_2H_2$ | C1s | 291.25 | 296.25 | | | 285.87 | 287.12 |
| CO | O1s | 542.10 | 547.89 | | | 534.28 | |

**Table S5:** Continued

| formula | core level | Ref | $G_0W_0$ | | | | |
|---|---|---|---|---|---|---|---|
| | | | HF | BLYP | PBE | B3LYP | PBE0 |
| CO | C1s | 296.23 | 300.51 | | | 290.92 | |
| $CO_2$ | O1s | 541.32 | 547.39 | | | 533.08 | 534.93 |
| $CO_2$ | C1s | 297.70 | 303.15 | | | 293.15 | 294.02 |
| $CF_4$ | F1s | 695.20 | 700.31 | | | 686.51 | 688.31 |
| $CF_4$ | C1s | 301.90 | 307.11 | | | 297.69 | 298.45 |
| $CFH_3$ | F1s | 692.40 | | | | 682.86 | 685.07 |
| $CFH_3$ | C1s | 293.56 | | | | 288.60 | 289.61 |
| $CF_3H$ | F1s | 694.10 | 700.65 | | | 684.95 | 687.02 |
| $CF_3H$ | C1s | 299.16 | 304.20 | | | 294.50 | 295.42 |
| $CH_3OH$ | O1s | 538.88 | 544.65 | | | | 532.81 |
| $CH_3OH$ | C1s | 292.30 | 297.27 | | | | 288.52 |
| $CH_2O$ | O1s | 539.33 | 545.20 | | | 530.50 | 532.47 |
| $CH_2O$ | C1s | 294.38 | 299.41 | | | 289.10 | 290.30 |
| $CH_3{-}O{-}CH_3$ | O1s | 538.36 | 544.37 | | | 529.97 | 532.14 |
| $CH_3{-}O{-}CH_3$ | C1s | 292.17 | 297.28 | | | 287.17 | 288.26 |
| HCOOH | O1s_OH | 540.69 | 546.59 | | | | 533.68 |
| HCOOH | O1s_C=O | 539.02 | 544.90 | | | | 531.69 |
| HCOOH | C1s | 295.75 | 300.90 | | | | 291.57 |
| $(CH_3)_2CO$ | O1s | 537.73 | 545.32 | | | 528.63 | 530.71 |
| $(CH_3)_2CO$ | C1s_C=O | 293.88 | 298.79 | | | 288.21 | 289.65 |
| $(CH_3)_2CO$ | C1s_CH3 | 291.23 | 296.09 | | | 285.98 | 287.24 |
| $CH_3CO_2H$ | O1s_OCH3 | 539.64 | 546.00 | | | | 533.11 |
| $CH_3CO_2H$ | O1s_C=O | 538.24 | 544.62 | | | | 531.19 |
| $CH_3COOH$ | O1s_OH | 540.10 | 546.18 | | | 531.05 | 533.15 |
| $CH_3COOH$ | O1s_C=O | 538.31 | 544.16 | | | 529.07 | 531.07 |
| $CH_3COOH$ | C1s_COOH | 295.35 | 300.54 | | | 290.00 | 291.41 |
| $CH_3COOH$ | C1s_CH3 | 291.55 | 296.47 | | | 286.61 | 287.64 |
| $H_2O$ | O1s | 539.70 | 545.07 | | | 531.53 | 533.71 |
| $O_3$ | O1s_midd | 546.44 | 554.57 | | | | 541.18 |
| $O_3$ | O1s_term | 541.75 | 548.78 | | | | 533.35 |
| $O_2$ | O1s_up | 544.20 | 550.28 | | | 535.99 | 537.32 |
| $O_2$ | O1s_down | 543.10 | 550.26 | | | 535.98 | 537.32 |

**Table S5:** Continued

| formula | core level | Ref | $G_0W_0$ | | | | |
|---|---|---|---|---|---|---|---|
| | | | HF | BLYP | PBE | B3LYP | PBE0 |
| $N_2$ | N1s | 409.93 | 415.15 | | | | 404.97 |
| $NH_3$ | N1s | 405.52 | 410.71 | | | 399.60 | 400.98 |
| HCN | N1s | 406.80 | 412.44 | | | | 401.41 |
| HCN | C1s | 293.50 | 297.95 | | | | 289.44 |
| $CH_3CN$ | N1s | 405.58 | 411.54 | | | 398.59 | |
| $CH_3CN$ | C1s_CH3 | 292.88 | 297.58 | | | 287.99 | |
| $CH_3CN$ | C1s_CN | 292.60 | 297.36 | | | 287.74 | |
| $C_2H_5NO_2$ | O1s_OH | 540.20 | 546.30 | | | | 533.27 |
| $C_2H_5NO_2$ | O1s_C=O | 538.40 | 545.80 | | | | 531.14 |
| $C_2H_5NO_2$ | N1s | 405.40 | 410.89 | | | | 400.97 |
| $C_2H_5NO_2$ | C1s_COOH | 295.20 | 300.48 | | | | 291.17 |
| $C_2H_5NO_2$ | C1s_CH2 | 292.30 | 297.28 | | | | 288.33 |
| $C_5H_5N$ | N1s | 404.82 | 410.79 | | | | 398.88 |
| $C_4H_4NH$ | N1s | 406.18 | 411.94 | | | 398.54 | 400.34 |
| $C_6H_5NH_2$ | N1s | 405.31 | 410.99 | | | | |
| $CO(NH_2)_2$ | O1s | 537.19 | 543.34 | | | | 529.79 |
| $CO(NH_2)_2$ | N1s | 406.09 | 411.65 | | | | 400.53 |
| $CO(NH_2)_2$ | C1s | 294.84 | 300.16 | | | | 290.95 |
| $CH_3NH_2$ | N1s | 405.17 | 410.47 | | | 398.52 | 399.86 |
| $C_6H_5NO_2$ | O1s | 538.63 | 545.53 | | | | |
| $C_6H_5NO_2$ | N1s | 411.60 | 418.82 | | | | |
| $C_6H_5NO_2$ | C1s_C1 | 292.08 | 297.59 | | | | |
| $C_6H_5NO_2$ | C1s_C234 | 291.13 | 296.76 | | | | |
| $C_6H_6$ | C1s | 290.38 | 295.65 | | | 284.16 | 285.48 |
| $C_8H_6$ | C1s_C3 | 290.88 | 296.37 | | | | |
| $C_8H_6$ | C1s_C2 | 290.55 | 295.89 | | | | |
| $C_8H_6$ | C1s_C456 | 290.16 | 295.80 | | | | |
| $C_8H_6$ | C1s_C1 | 289.75 | 295.58 | | | | |

**Table S6:** Core-level of the CORE65 set[S3] obtained from ev$GW_0$ and ev$GW$ with HF, BLYP, PBE, B3LYP and PBE0. The cc-pVTZ basis set was used. All values in eV.

| | | | ev$GW_0$ | | | | | ev$GW$ | | | | |
|---|---|---|---|---|---|---|---|---|---|---|---|---|
| formula | core level | Ref | HF | BLYP | PBE | B3LYP | PBE0 | HF | BLYP | PBE | B3LYP | PBE0 |
| $CH_4$ | C1s | 290.84 | 294.05 | 289.58 | 289.72 | 290.43 | 290.89 | 293.74 | 291.53 | 291.72 | 291.83 | 292.11 |
| $C_2H_6$ | C1s | 290.71 | 294.00 | 289.39 | 289.36 | 290.33 | 290.83 | 293.65 | 291.39 | 291.63 | 291.73 | 292.03 |
| $C_2H_4$ | C1s | 290.82 | 294.33 | 289.17 | 289.68 | 290.64 | 291.16 | 293.95 | 291.87 | 292.02 | 292.08 | 292.34 |
| $C_2H_2$ | C1s | 291.25 | 294.69 | 289.70 | 289.72 | 291.14 | 290.82 | 294.35 | 292.07 | 292.32 | 292.44 | 292.76 |
| CO | O1s | 542.10 | 545.27 | 540.60 | 540.97 | | 541.49 | 544.72 | 543.11 | 543.57 | 543.33 | 543.87 |
| CO | C1s | 296.23 | 299.37 | 294.81 | 294.88 | | 296.00 | 299.08 | 296.56 | 296.72 | 297.04 | 297.26 |
| $CO_2$ | O1s | 541.32 | 544.64 | 539.21 | 540.24 | 540.37 | 539.84 | 543.95 | 541.84 | 542.33 | 542.19 | 542.72 |
| $CO_2$ | C1s | 297.70 | 301.97 | 296.03 | 296.02 | 297.25 | 297.62 | 301.44 | 297.89 | 297.90 | 298.57 | 298.76 |
| $CF_4$ | F1s | 695.20 | 698.45 | | 692.96 | 693.46 | 694.58 | 697.72 | 695.92 | 696.34 | 696.19 | 696.62 |
| $CF_4$ | C1s | 301.90 | 306.05 | | 299.78 | 301.34 | 301.67 | 305.53 | 301.90 | 301.85 | 302.69 | 302.79 |
| $CFH_3$ | F1s | 692.40 | 697.31 | 691.12 | 690.96 | 690.53 | 691.97 | 694.69 | 693.22 | 693.71 | 693.40 | 693.89 |
| $CFH_3$ | C1s | 293.56 | 297.03 | 292.24 | 292.32 | 293.15 | 293.58 | 296.66 | 294.16 | 294.28 | 294.55 | 294.89 |
| $CF_3H$ | F1s | 694.10 | 697.03 | 691.77 | 692.10 | 692.63 | 693.49 | 696.64 | 694.98 | 695.44 | 695.23 | 695.69 |
| $CF_3H$ | C1s | 299.16 | 303.13 | 297.19 | 297.03 | 298.66 | 299.04 | 302.63 | 299.38 | 299.43 | 300.01 | 300.19 |
| $CH_3OH$ | O1s | 538.88 | 542.04 | 536.09 | 537.54 | 537.90 | 538.72 | 541.46 | 539.49 | 540.00 | 539.77 | 540.32 |
| $CH_3OH$ | C1s | 292.30 | 295.87 | 291.09 | 291.25 | 292.02 | 292.51 | 295.48 | 293.10 | 293.27 | 293.46 | 293.71 |
| $CH_2O$ | O1s | 539.33 | 542.38 | 537.41 | 537.72 | 538.54 | 539.35 | 541.82 | 540.05 | 540.55 | 540.30 | 540.83 |
| $CH_2O$ | C1s | 294.38 | 298.11 | 292.95 | 292.72 | 294.32 | 294.35 | 297.73 | 295.17 | 295.31 | 295.59 | 295.83 |
| $CH_3{-}O{-}CH_3$ | O1s | 538.36 | 541.50 | 536.90 | 537.13 | 537.30 | 538.31 | 540.88 | 538.96 | 539.56 | 539.25 | 539.85 |
| $CH_3{-}O{-}CH_3$ | C1s | 292.17 | 295.71 | 290.86 | 290.88 | 291.84 | 292.31 | 295.27 | 292.86 | 293.04 | 293.22 | 293.47 |
| HCOOH | O1s_OH | 540.69 | 543.91 | 538.24 | 538.09 | 539.70 | 540.02 | 543.24 | 541.14 | 541.63 | 541.45 | 541.99 |
| HCOOH | O1s_C=O | 539.02 | 542.06 | 536.56 | 537.04 | 538.08 | 538.47 | 541.37 | 539.42 | 539.90 | 539.72 | 540.24 |
| HCOOH | C1s | 295.75 | 299.67 | 294.15 | 294.09 | 295.31 | 295.75 | 299.26 | 296.15 | 296.19 | 296.70 | 296.91 |
| $(CH_3)_2CO$ | O1s | 537.73 | 541.74 | 535.77 | 536.02 | 537.03 | 537.62 | 540.45 | 538.46 | 538.94 | 538.77 | 539.30 |
| $(CH_3)_2CO$ | C1s_C=O | 293.88 | 297.35 | 292.04 | 291.95 | 293.36 | 293.94 | 296.87 | 294.21 | 294.40 | 294.68 | 295.01 |
| $(CH_3)_2CO$ | C1s_CH3 | 291.23 | 294.60 | 289.85 | 290.06 | 290.81 | 291.29 | 294.13 | 291.78 | 291.98 | 292.15 | 292.45 |
| $CH_3CO_2H$ | O1s_OCH3 | 539.64 | 543.12 | 537.70 | 538.07 | 538.95 | 539.71 | 542.37 | 540.34 | 540.92 | 540.66 | 541.26 |
| $CH_3CO_2H$ | O1s_C=O | 538.24 | 541.72 | 536.25 | 536.50 | 537.63 | 538.35 | 540.96 | 538.94 | 539.43 | 539.27 | 539.81 |
| $CH_3COOH$ | O1s_OH | 540.10 | 543.45 | 537.51 | 538.21 | 539.11 | 539.84 | 542.75 | 540.51 | 540.99 | 540.85 | 541.39 |
| $CH_3COOH$ | O1s_C=O | 538.31 | 541.64 | 536.00 | 536.46 | 537.37 | 538.09 | 540.76 | 538.73 | 539.19 | 539.07 | 539.60 |
| $CH_3COOH$ | C1s_COOH | 295.35 | 299.24 | 293.50 | 293.87 | 294.85 | 295.36 | 298.74 | 295.62 | 295.76 | 296.22 | 296.49 |

**Table S6:** Continued

| | | | ev$GW_0$ | | | | | ev$GW$ | | | | |
|---|---|---|---|---|---|---|---|---|---|---|---|---|
| formula | core level | Ref | HF | BLYP | PBE | B3LYP | PBE0 | HF | BLYP | PBE | B3LYP | PBE0 |
| $CH_3COOH$ | C1s_CH3 | 291.55 | 295.02 | 290.13 | 290.38 | 291.21 | 291.69 | 294.57 | 292.21 | 292.41 | 292.57 | 292.86 |
| $H_2O$ | O1s | 539.70 | 542.67 | 536.72 | 536.60 | 538.69 | 539.42 | 542.20 | 540.30 | 540.73 | 540.54 | 541.03 |
| $O_3$ | O1s_midd | 546.44 | 551.86 | 545.58 | 545.74 | 546.54 | | 551.08 | 547.54 | 548.04 | 548.20 | 548.80 |
| $O_3$ | O1s_term | 541.75 | 545.78 | 539.46 | 539.33 | 540.99 | | 545.12 | 542.45 | 542.86 | 542.99 | 543.45 |
| $O_2$ | O1s_up | 544.20 | 547.86 | | | 543.57 | 544.31 | 547.35 | | | 545.31 | 545.80 |
| $O_2$ | O1s_down | 543.10 | 547.84 | | | 543.55 | 544.29 | 547.33 | | | 545.29 | 545.78 |
| $N_2$ | N1s | 409.93 | 413.33 | 408.07 | 408.16 | 408.45 | 409.63 | 412.95 | 410.47 | 410.79 | 410.91 | 411.29 |
| $NH_3$ | N1s | 405.52 | 408.72 | 404.00 | 404.31 | 404.79 | 405.46 | 408.34 | 406.12 | 406.50 | 406.43 | 406.87 |
| HCN | N1s | 406.80 | 410.26 | 403.82 | 405.70 | 406.44 | 406.13 | 409.82 | 407.51 | 407.91 | 407.88 | 408.35 |
| HCN | C1s | 293.50 | 296.93 | 291.30 | 291.00 | 292.18 | 293.26 | 296.32 | 294.03 | 294.21 | 294.41 | 294.67 |
| $CH_3CN$ | N1s | 405.58 | 409.23 | 403.69 | 404.59 | 404.55 | 404.74 | 408.75 | 406.25 | 406.65 | 406.66 | 407.13 |
| $CH_3CN$ | C1s_CH3 | 292.88 | 296.14 | 291.35 | 291.72 | 292.36 | 292.83 | 295.73 | 293.33 | 293.54 | 293.71 | 294.01 |
| $CH_3CN$ | C1s_CN | 292.60 | 295.91 | 290.76 | 290.43 | 292.36 | 292.49 | 295.57 | 293.17 | 293.38 | 293.60 | 293.89 |
| $C_2H_5NO_2$ | O1s_OH | 540.20 | 543.55 | 537.81 | 538.52 | 539.15 | 539.69 | 542.81 | 540.52 | 541.01 | 540.88 | 541.42 |
| $C_2H_5NO_2$ | O1s_C=O | 538.40 | 541.89 | 536.09 | 536.66 | 537.38 | 538.02 | 540.84 | 538.79 | 539.26 | 539.13 | 539.65 |
| $C_2H_5NO_2$ | N1s | 405.40 | 408.79 | 403.68 | 404.16 | 404.54 | 405.40 | 408.21 | 405.90 | 406.33 | 406.26 | 406.76 |
| $C_2H_5NO_2$ | C1s_COOH | 295.20 | 299.12 | 293.46 | 293.63 | 294.72 | 295.17 | 298.61 | 295.39 | 295.50 | 295.95 | 296.25 |
| $C_2H_5NO_2$ | C1s_CH2 | 292.30 | 295.81 | 290.84 | 290.98 | 291.90 | 292.40 | 295.33 | 292.82 | 293.03 | 293.23 | 293.54 |
| $C_5H_5N$ | N1s | 404.82 | 408.26 | 403.08 | 403.41 | 404.25 | 404.91 | 407.62 | 405.19 | 405.67 | 405.63 | 406.16 |
| $C_4H_4NH$ | N1s | 406.18 | 409.54 | 404.19 | 404.27 | 405.07 | 406.23 | 408.88 | 406.62 | 407.12 | 406.98 | 407.55 |
| $C_6H_5NH_2$ | N1s | 405.31 | 408.67 | 403.35 | 404.05 | 404.49 | 405.27 | 408.00 | 405.66 | 406.12 | 406.02 | 406.53 |
| $CO(NH_2)_2$ | O1s | 537.19 | 540.36 | 534.84 | 535.57 | 535.75 | 536.81 | 539.55 | 537.51 | 538.00 | 537.81 | 538.35 |
| $CO(NH_2)_2$ | N1s | 406.09 | 409.53 | 404.23 | 404.87 | 405.33 | 406.09 | 408.94 | 406.52 | 406.94 | 406.90 | 407.40 |
| $CO(NH_2)_2$ | C1s | 294.84 | 298.86 | 293.18 | 293.24 | 294.42 | 294.88 | 298.41 | 295.18 | 295.31 | 295.79 | 296.04 |
| $CH_3NH_2$ | N1s | 405.17 | 408.37 | 403.86 | 404.15 | 404.41 | 405.12 | 407.88 | 405.66 | 406.10 | 406.00 | 406.50 |
| $C_6H_5NO_2$ | O1s | 538.63 | 542.95 | 535.86 | 537.15 | 537.85 | 538.71 | 541.50 | 539.06 | 539.57 | 539.51 | 540.08 |
| $C_6H_5NO_2$ | N1s | 411.60 | 416.93 | 409.49 | 410.13 | 411.23 | 411.93 | 415.95 | 411.83 | 412.24 | 412.61 | 413.29 |
| $C_6H_5NO_2$ | C1s_C1 | 292.08 | 295.85 | 290.48 | 291.09 | 291.64 | 292.31 | 295.25 | 292.52 | 292.86 | 293.07 | 293.42 |
| $C_6H_5NO_2$ | C1s_C234 | 291.13 | 294.97 | 289.68 | 290.17 | 290.86 | 291.36 | 294.41 | 291.72 | 291.99 | 292.17 | 292.53 |
| $C_6H_6$ | C1s | 290.38 | 293.85 | 288.77 | 289.42 | 289.98 | 290.52 | 293.34 | 290.97 | 291.26 | 291.44 | 291.58 |
| $C_8H_6$ | C1s_C3 | 290.88 | 294.59 | 289.73 | 290.07 | 290.70 | 291.39 | 293.99 | 291.62 | 291.92 | 292.00 | 292.38 |
| $C_8H_6$ | C1s_C2 | 290.55 | 294.06 | 288.85 | 289.46 | 290.11 | 290.68 | 293.48 | 290.98 | 291.26 | 291.39 | 291.77 |

**Table S6:** Continued

| formula | core level | Ref | ev$GW_0$ HF | ev$GW_0$ BLYP | ev$GW_0$ PBE | ev$GW_0$ B3LYP | ev$GW_0$ PBE0 | ev$GW$ HF | ev$GW$ BLYP | ev$GW$ PBE | ev$GW$ B3LYP | ev$GW$ PBE0 |
|---|---|---|---|---|---|---|---|---|---|---|---|---|
| $C_8H_6$ | C1s_C456 | 290.16 | 294.07 | 289.25 | 289.38 | 290.11 | 290.95 | 293.60 | 291.17 | 291.45 | 291.57 | 291.95 |
| $C_8H_6$ | C1s_C1 | 289.75 | 293.85 | 288.52 | 289.02 | 289.86 | 289.99 | 293.30 | 290.76 | 291.04 | 291.20 | 291.57 |

**Table S7:** Core-level of the CORE65 set[S3] obtained from $G_{\mathrm{RS}}W_0$ and $G_{\mathrm{RS}}W_{\mathrm{RS}}$ with HF, BLYP, PBE, B3LYP and PBE0. The cc-pVTZ basis set was used. All values in eV.

| formula | core level | Ref | $G_{\mathrm{RS}}W_0$ HF | $G_{\mathrm{RS}}W_0$ BLYP | $G_{\mathrm{RS}}W_0$ PBE | $G_{\mathrm{RS}}W_0$ B3LYP | $G_{\mathrm{RS}}W_0$ PBE0 | $G_{\mathrm{RS}}W_{\mathrm{RS}}$ HF | $G_{\mathrm{RS}}W_{\mathrm{RS}}$ BLYP | $G_{\mathrm{RS}}W_{\mathrm{RS}}$ PBE | $G_{\mathrm{RS}}W_{\mathrm{RS}}$ B3LYP | $G_{\mathrm{RS}}W_{\mathrm{RS}}$ PBE0 |
|---|---|---|---|---|---|---|---|---|---|---|---|---|
| $CH_4$ | C1s | 290.84 | 295.48 | 292.33 | 292.43 | 292.83 | 293.18 | 295.48 | 293.58 | 293.74 | 293.84 | 294.06 |
| $C_2H_6$ | C1s | 290.71 | 295.49 | 292.21 | 292.42 | 292.83 | 293.20 | 295.49 | 293.63 | 293.82 | 293.89 | 294.14 |
| $C_2H_4$ | C1s | 290.82 | 295.90 | 292.58 | 293.16 | 293.30 | 293.65 | 295.90 | 293.70 | 294.26 | 294.34 | 294.55 |
| $C_2H_2$ | C1s | 291.25 | 296.25 | 293.39 | 293.55 | 293.64 | 294.07 | 296.25 | 294.27 | 294.50 | 294.58 | 294.88 |
| CO | O1s | 542.10 | 547.89 | | 545.17 | | 546.34 | 547.89 | 546.63 | 547.06 | 546.81 | 547.25 |
| CO | C1s | 296.23 | 300.51 | | 296.57 | | 297.81 | 300.51 | 298.28 | 298.41 | 298.68 | 298.89 |
| $CO_2$ | O1s | 541.32 | 547.39 | 544.15 | | | 544.96 | 547.38 | 545.71 | 546.13 | 545.99 | 546.43 |
| $CO_2$ | C1s | 297.70 | 303.15 | 298.31 | | | 299.41 | 303.15 | 299.59 | 299.60 | 300.24 | 300.40 |
| $CF_4$ | F1s | 695.20 | 700.31 | 696.78 | 698.16 | 698.29 | 698.71 | 700.31 | 699.20 | 699.55 | 699.37 | 699.71 |
| $CF_4$ | C1s | 301.90 | 307.11 | 302.15 | 302.07 | 303.29 | 303.43 | 307.11 | 303.69 | 303.67 | 304.42 | 304.53 |
| $CFH_3$ | F1s | 692.40 | | 695.00 | 694.77 | 696.03 | 696.62 | | 696.53 | 696.91 | 696.56 | 696.92 |
| $CFH_3$ | C1s | 293.56 | | 294.89 | 294.95 | 295.45 | 295.78 | | 296.20 | 296.32 | 296.53 | 296.73 |
| $CF_3H$ | F1s | 694.10 | 700.65 | 697.02 | 697.74 | 697.70 | 697.91 | 700.65 | 698.30 | 698.57 | 698.39 | 698.63 |
| $CF_3H$ | C1s | 299.16 | 304.20 | 299.66 | 299.47 | 300.70 | 300.97 | 304.20 | 301.23 | 301.26 | 301.82 | 301.96 |
| $CH_3OH$ | O1s | 538.88 | 544.65 | 541.64 | 542.33 | 542.09 | | 544.65 | 543.17 | 543.64 | 543.35 | 543.84 |
| $CH_3OH$ | C1s | 292.30 | 297.27 | 293.72 | 294.05 | 294.44 | | 297.27 | 295.26 | 295.39 | 295.54 | 295.74 |
| $CH_2O$ | O1s | 539.33 | 545.20 | 541.08 | 543.58 | | 543.43 | 545.20 | 543.90 | 544.35 | 544.06 | 544.52 |
| $CH_2O$ | C1s | 294.38 | 299.41 | 295.76 | 295.59 | | 296.85 | 299.41 | 297.14 | 297.24 | 297.50 | 297.70 |
| $CH_3{-}O{-}CH_3$ | O1s | 538.36 | 544.37 | 541.34 | 541.24 | 541.98 | 542.59 | 544.37 | 543.08 | 543.60 | 543.23 | 543.75 |
| $CH_3{-}O{-}CH_3$ | C1s | 292.17 | 297.28 | 293.76 | 293.88 | 294.33 | 294.65 | 297.28 | 295.08 | 295.22 | 295.36 | 295.57 |
| HCOOH | O1s_OH | 540.69 | 546.59 | | | 543.93 | 544.55 | 546.58 | 545.02 | 545.47 | 545.23 | 545.70 |
| HCOOH | O1s_C=O | 539.02 | 544.90 | | | 542.48 | 543.07 | 544.90 | 543.45 | 543.88 | 543.67 | 544.12 |
| HCOOH | C1s | 295.75 | 300.90 | | | 297.47 | 297.84 | 300.90 | 298.11 | 298.18 | 298.62 | 298.81 |
| $(CH_3)_2CO$ | O1s | 537.73 | 545.32 | 541.33 | | 541.47 | 542.34 | 545.32 | 542.36 | 542.78 | 542.52 | 542.92 |

**Table S7:** Continued

| formula | core level | Ref | $G_{\mathrm{RS}}W_0$ | | | | | $G_{\mathrm{RS}}W_{\mathrm{RS}}$ | | | | |
|---|---|---|---|---|---|---|---|---|---|---|---|---|
| | | | HF | BLYP | PBE | B3LYP | PBE0 | HF | BLYP | PBE | B3LYP | PBE0 |
| $(CH_3)_2CO$ | C1s_C=O | 293.88 | 298.79 | 294.99 | | 295.79 | 296.18 | 298.79 | 296.45 | 296.61 | 296.83 | 297.13 |
| $(CH_3)_2CO$ | C1s_CH3 | 291.23 | 296.09 | 292.81 | | 293.35 | 293.73 | 296.09 | 294.09 | 294.27 | 294.38 | 294.64 |
| $CH_3CO_2H$ | O1s_OCH3 | 539.64 | 546.00 | 543.03 | | 543.47 | 544.25 | 546.00 | 544.63 | 545.11 | 544.81 | 545.31 |
| $CH_3CO_2H$ | O1s_C=O | 538.24 | 544.62 | 541.46 | | 541.88 | 542.62 | 544.62 | 543.16 | 543.60 | 543.38 | 543.84 |
| $CH_3COOH$ | O1s_OH | 540.10 | 546.18 | 543.17 | 543.76 | 543.56 | 544.09 | 546.18 | 544.55 | 545.00 | 544.78 | 545.25 |
| $CH_3COOH$ | O1s_C=O | 538.31 | 544.16 | 540.80 | 542.23 | 541.94 | 542.47 | 544.15 | 542.86 | 543.27 | 543.05 | 543.48 |
| $CH_3COOH$ | C1s_COOH | 295.35 | 300.54 | 296.28 | 296.61 | 297.21 | 297.50 | 300.54 | 297.77 | 297.87 | 298.25 | 298.50 |
| $CH_3COOH$ | C1s_CH3 | 291.55 | 296.47 | 293.08 | 293.49 | 293.70 | 294.03 | 296.47 | 294.44 | 294.61 | 294.75 | 294.99 |
| $H_2O$ | O1s | 539.70 | 545.07 | | 542.67 | 542.10 | 542.96 | 545.07 | 543.52 | 543.92 | 543.71 | 544.14 |
| $O_3$ | O1s_midd | 546.44 | 554.57 | 549.31 | | 550.62 | 551.45 | 554.57 | 551.37 | 551.82 | 551.95 | 552.50 |
| $O_3$ | O1s_term | 541.75 | 548.78 | 545.18 | | 545.89 | 546.47 | 548.78 | 546.47 | 546.85 | 546.93 | 547.36 |
| $O_2$ | O1s_up | 544.20 | 550.28 | | | | 547.89 | 550.28 | | | 548.54 | 548.96 |
| $O_2$ | O1s_down | 543.10 | 550.26 | | | | 547.88 | 550.26 | | | 548.52 | 548.94 |
| $N_2$ | N1s | 409.93 | 415.15 | 411.22 | 411.34 | 412.41 | 412.95 | 415.15 | 412.96 | 413.25 | 413.34 | 413.69 |
| $NH_3$ | N1s | 405.52 | 410.71 | 407.64 | 407.90 | 407.87 | 408.48 | 410.71 | 408.86 | 409.21 | 409.10 | 409.50 |
| HCN | N1s | 406.80 | 412.44 | 408.19 | 409.97 | 409.88 | 410.31 | 412.44 | 410.43 | 410.79 | 410.75 | 411.16 |
| HCN | C1s | 293.50 | 297.95 | 294.98 | 295.06 | 295.33 | 295.70 | 297.95 | 295.80 | 295.93 | 296.05 | 296.19 |
| $CH_3CN$ | N1s | 405.58 | 411.54 | | 408.99 | 408.71 | 409.29 | 411.54 | 409.28 | 409.55 | 409.57 | 409.80 |
| $CH_3CN$ | C1s_CH3 | 292.88 | 297.58 | | 294.49 | 294.82 | 295.10 | 297.58 | 295.53 | 295.68 | 295.78 | 296.12 |
| $CH_3CN$ | C1s_CN | 292.60 | 297.36 | | 294.33 | 294.69 | 295.14 | 297.36 | 295.27 | 295.44 | 295.61 | 295.92 |
| $C_2H_5NO_2$ | O1s_OH | 540.20 | 546.30 | 543.28 | 543.62 | 543.66 | 544.16 | 546.30 | 544.64 | 545.07 | 544.88 | 545.34 |
| $C_2H_5NO_2$ | O1s_C=O | 538.40 | 545.80 | 541.60 | 542.05 | 542.01 | 542.70 | 545.81 | 542.61 | 542.77 | 542.64 | 542.74 |
| $C_2H_5NO_2$ | N1s | 405.40 | 410.89 | 407.51 | 407.94 | 408.15 | 408.67 | 410.89 | 409.02 | 409.43 | 409.30 | 409.74 |
| $C_2H_5NO_2$ | C1s_COOH | 295.20 | 300.48 | 296.15 | 296.12 | 297.02 | 297.40 | 300.48 | 297.58 | 297.69 | 298.12 | 298.32 |
| $C_2H_5NO_2$ | C1s_CH2 | 292.30 | 297.28 | 293.66 | 294.21 | 294.38 | 294.76 | 297.28 | 295.06 | 295.18 | 295.40 | 295.77 |
| $C_5H_5N$ | N1s | 404.82 | 410.79 | 407.39 | 408.50 | 407.77 | 408.79 | 410.79 | 408.81 | 409.26 | 409.13 | 409.62 |
| $C_4H_4NH$ | N1s | 406.18 | 411.94 | 408.95 | 409.25 | 409.43 | 410.07 | 411.94 | 410.12 | 410.58 | 410.40 | 410.90 |
| $C_6H_5NH_2$ | N1s | 405.31 | 410.99 | 408.01 | 408.50 | 408.46 | 408.96 | 410.98 | 409.24 | 409.67 | 409.48 | 409.93 |
| $CO(NH_2)_2$ | O1s | 537.19 | 543.34 | | 541.17 | 540.29 | 541.21 | 543.34 | 541.90 | 542.33 | 542.12 | 542.54 |
| $CO(NH_2)_2$ | N1s | 406.09 | 411.66 | | 408.84 | 408.82 | 409.37 | 411.65 | 409.68 | 410.14 | 409.98 | 410.44 |
| $CO(NH_2)_2$ | C1s | 294.84 | 300.16 | | 295.83 | 296.72 | 297.05 | 300.16 | 297.21 | 297.30 | 297.76 | 297.98 |
| $CH_3NH_2$ | N1s | 405.17 | 410.47 | 407.29 | 407.64 | 407.80 | 408.28 | 410.47 | 408.67 | 409.07 | 408.92 | 409.36 |

**Table S7:** Continued

| formula | core level | Ref | $G_{RS}W_0$ HF | BLYP | PBE | B3LYP | PBE0 | $G_{RS}W_{RS}$ HF | BLYP | PBE | B3LYP | PBE0 |
|---|---|---|---|---|---|---|---|---|---|---|---|---|
| $C_6H_5NO_2$ | O1s | 538.63 | 545.53 | 542.28 | 543.33 | 543.11 | 543.71 | 545.53 | 543.77 | 544.21 | 544.10 | 544.58 |
| $C_6H_5NO_2$ | N1s | 411.60 | 418.82 | 414.00 | 414.13 | 414.81 | 415.11 | 418.83 | 415.21 | 415.63 | 415.91 | 416.46 |
| $C_6H_5NO_2$ | C1s_C1 | 292.08 | 297.59 | 294.13 | 294.34 | 294.80 | 295.27 | 297.59 | 295.33 | 295.59 | 295.73 | 296.04 |
| $C_6H_5NO_2$ | C1s_C234 | 291.13 | 296.76 | 293.40 | 293.54 | 293.92 | 294.36 | 296.79 | 294.50 | 294.76 | 294.88 | 295.18 |
| $C_6H_6$ | C1s | 290.38 | 295.65 | 292.63 | 292.84 | 293.04 | 293.47 | 295.65 | 293.66 | 293.91 | 293.97 | 294.29 |
| $C_8H_6$ | C1s_C3 | 290.88 | 296.37 | 293.17 | 293.48 | 293.66 | 294.22 | 296.37 | 294.32 | 294.58 | 294.64 | 295.00 |
| $C_8H_6$ | C1s_C2 | 290.55 | 295.89 | 292.65 | 293.00 | 293.22 | 293.68 | 295.89 | 293.82 | 294.07 | 294.15 | 294.48 |
| $C_8H_6$ | C1s_C456 | 290.16 | 295.80 | 292.69 | 292.86 | 293.29 | 293.71 | 295.80 | 293.76 | 294.07 | 294.14 | 294.44 |
| $C_8H_6$ | C1s_C1 | 289.75 | 295.58 | 292.66 | 292.83 | 293.04 | 293.45 | 295.58 | 293.45 | 293.64 | 293.72 | 293.92 |

**Table S8:** Core-level of the CORE65 set[S3] obtained from $G_{RSc}W_0$ and $G_{RSc}W_{RSc}$ with HF, BLYP, PBE, B3LYP and PBE0. The cc-pVTZ basis set was used. All values in eV.

| formula | core level | Ref | $G_{RSc}W_0$ HF | BLYP | PBE | B3LYP | PBE0 | $G_{RSc}W_{RSc}$ HF | BLYP | PBE | B3LYP | PBE0 |
|---|---|---|---|---|---|---|---|---|---|---|---|---|
| $CH_4$ | C1s | 290.84 | 294.35 | 290.54 | 290.68 | 291.19 | 291.59 | 294.14 | 291.90 | 292.08 | 292.21 | 292.48 |
| $C_2H_6$ | C1s | 290.71 | 294.29 | 290.40 | 290.68 | 291.15 | 291.57 | 294.05 | 291.83 | 292.04 | 292.16 | 292.45 |
| $C_2H_4$ | C1s | 290.82 | 294.64 | 290.91 | 291.41 | 291.52 | 291.94 | 294.38 | 292.08 | 292.34 | 292.44 | 292.77 |
| $C_2H_2$ | C1s | 291.25 | 295.01 | 291.75 | 291.75 | 291.92 | 292.41 | 294.78 | 292.46 | 292.71 | 292.82 | 293.14 |
| CO | O1s | 542.10 | 545.82 | 542.14 | 542.96 | 543.09 | 543.90 | 545.47 | 543.86 | 544.32 | 544.10 | 544.57 |
| CO | C1s | 296.23 | 299.56 | 295.56 | 295.64 | 297.10 | 296.57 | 299.37 | 296.87 | 297.01 | 297.30 | 297.54 |
| $CO_2$ | O1s | 541.32 | 545.20 | 541.38 | 541.67 | 542.36 | 542.57 | 544.77 | 542.66 | 543.13 | 543.02 | 543.51 |
| $CO_2$ | C1s | 297.70 | 302.15 | 296.79 | 296.78 | 297.84 | 298.16 | 301.82 | 298.12 | 298.15 | 298.81 | 298.99 |
| $CF_4$ | F1s | 695.20 | 700.25 | 695.12 | 695.54 | 695.59 | 695.77 | 698.69 | 696.64 | 697.00 | 697.21 | 697.51 |
| $CF_4$ | C1s | 301.90 | 306.32 | 300.63 | 300.58 | 301.92 | 302.19 | 305.84 | 302.17 | 302.16 | 302.95 | 303.09 |
| $CFH_3$ | F1s | 692.40 |  | 691.94 | 694.09 | 692.73 | 693.12 |  | 693.97 | 694.42 | 694.12 | 694.57 |
| $CFH_3$ | C1s | 293.56 |  | 293.19 | 293.27 | 293.87 | 294.25 |  | 294.71 | 294.65 | 294.99 | 295.17 |
| $CF_3H$ | F1s | 694.10 | 697.47 | 693.36 | 694.25 | 694.54 | 694.96 | 697.53 | 695.76 | 696.16 | 696.00 | 696.41 |
| $CF_3H$ | C1s | 299.16 | 303.31 | 298.09 | 298.00 | 299.29 | 299.59 | 302.91 | 299.68 | 299.75 | 300.36 | 300.52 |
| $CH_3OH$ | O1s | 538.88 | 542.58 | 538.68 | 539.27 | 539.37 | 539.96 | 542.18 | 540.30 | 540.80 | 540.57 | 541.10 |
| $CH_3OH$ | C1s | 292.30 | 296.13 | 292.03 | 292.16 | 292.86 | 293.19 | 295.84 | 293.51 | 293.67 | 293.86 | 294.11 |
| $CH_2O$ | O1s | 539.33 | 543.00 | 540.95 | 540.79 | 539.97 | 540.67 | 542.63 | 540.92 | 541.40 | 541.16 | 541.66 |

**Table S8:** Continued

| formula | core level | Ref | $G_{\mathrm{RSc}}W_0$ HF | BLYP | PBE | B3LYP | PBE0 | $G_{\mathrm{RSc}}W_{\mathrm{RSc}}$ HF | BLYP | PBE | B3LYP | PBE0 |
|---|---|---|---|---|---|---|---|---|---|---|---|---|
| $CH_2O$ | C1s | 294.38 | 298.34 | 295.61 | 295.11 | 295.00 | 295.40 | 298.07 | 295.55 | 295.68 | 295.96 | 296.20 |
| $CH_3{-}O{-}CH_3$ | O1s | 538.36 | 542.09 | 538.45 | 538.92 | 539.10 | 539.66 | 541.74 | 539.95 | 540.50 | 540.20 | 540.77 |
| $CH_3{-}O{-}CH_3$ | C1s | 292.17 | 295.98 | 291.83 | 292.09 | 292.64 | 293.04 | 295.67 | 293.31 | 293.48 | 293.66 | 293.91 |
| HCOOH | O1s_OH | 540.69 | 544.47 | 540.89 | 540.93 | 541.09 | 541.79 | 544.02 | 542.02 | 542.50 | 542.31 | 542.82 |
| HCOOH | O1s_C=O | 539.02 | 542.68 | 539.52 | 540.05 | 539.55 | 540.45 | 542.23 | 540.35 | 540.82 | 540.65 | 541.15 |
| HCOOH | C1s | 295.75 | 299.87 | 295.07 | 295.07 | 296.01 | 296.36 | 299.53 | 296.47 | 296.54 | 297.04 | 297.27 |
| $(CH_3)_2CO$ | O1s | 537.73 | 542.42 | 538.27 | 538.66 | 538.60 | 539.34 | 541.64 | 539.41 | 539.88 | 539.69 | 540.18 |
| $(CH_3)_2CO$ | C1s_C=O | 293.88 | 297.62 | 293.11 | 293.98 | 294.14 | 294.61 | 297.28 | 294.64 | 294.84 | 295.11 | 295.42 |
| $(CH_3)_2CO$ | C1s_CH3 | 291.23 | 294.90 | 291.00 | 291.12 | 291.63 | 292.04 | 294.56 | 292.27 | 292.47 | 292.62 | 292.90 |
| $CH_3CO_2H$ | O1s_OCH3 | 539.64 | 543.75 | 540.28 | 540.36 | 540.68 | 541.13 | 543.24 | 541.37 | 541.91 | 541.64 | 542.21 |
| $CH_3CO_2H$ | O1s_C=O | 538.24 | 542.36 | 538.87 | 538.76 | 539.32 | 539.81 | 541.85 | 539.95 | 540.43 | 540.25 | 540.77 |
| $CH_3COOH$ | O1s_OH | 540.10 | 544.04 | 540.04 | 540.75 | 540.57 | 541.33 | 543.56 | 541.45 | 541.93 | 541.77 | 542.29 |
| $CH_3COOH$ | O1s_C=O | 538.31 | 542.10 | 538.40 | 539.45 | 538.92 | 539.66 | 541.62 | 539.71 | 540.14 | 539.99 | 540.46 |
| $CH_3COOH$ | C1s_COOH | 295.35 | 299.47 | 294.58 | 294.77 | 295.71 | 296.01 | 299.12 | 296.00 | 296.13 | 296.65 | 296.88 |
| $CH_3COOH$ | C1s_CH3 | 291.55 | 295.29 | 291.38 | 291.37 | 292.01 | 292.42 | 294.96 | 292.65 | 292.84 | 293.01 | 293.29 |
| $H_2O$ | O1s | 539.70 | 543.15 | 539.95 | 540.13 | 539.85 | 540.50 | 542.83 | 540.92 | 541.35 | 541.19 | 541.66 |
| $O_3$ | O1s_midd | 546.44 | 552.41 | 547.24 | 547.47 | 547.93 | 548.88 | 551.91 | 548.40 | 548.90 | 549.05 | 549.65 |
| $O_3$ | O1s_term | 541.75 | 546.45 | 541.97 | 542.44 | 542.90 | 543.60 | 546.04 | 543.46 | 543.87 | 543.96 | 544.44 |
| $O_2$ | O1s_up | 544.20 | 548.33 | | | 544.78 | 545.46 | 547.99 | | | 545.99 | 546.46 |
| $O_2$ | O1s_down | 543.10 | 548.32 | | | 544.77 | 545.44 | 547.97 | | | 545.98 | 546.45 |
| $N_2$ | N1s | 409.93 | 413.67 | 411.10 | 410.78 | 410.58 | 411.85 | 413.40 | 410.93 | 411.25 | 411.37 | 411.74 |
| $NH_3$ | N1s | 405.52 | 409.13 | 405.22 | 405.68 | 405.80 | 406.39 | 408.87 | 406.66 | 407.03 | 406.97 | 407.41 |
| HCN | N1s | 406.80 | 410.73 | 406.72 | 408.68 | 407.47 | 408.19 | 410.44 | 408.10 | 408.49 | 408.48 | 408.92 |
| HCN | C1s | 293.50 | 297.08 | 293.47 | 293.45 | 293.81 | 294.46 | 296.66 | 294.33 | 294.51 | 294.70 | 294.94 |
| $CH_3CN$ | N1s | 405.58 | 409.72 | 405.65 | 407.23 | 406.32 | 407.24 | 409.40 | 406.87 | 407.24 | 407.31 | 407.73 |
| $CH_3CN$ | C1s_CH3 | 292.88 | 296.40 | 292.32 | 292.71 | 293.12 | 293.57 | 296.11 | 293.77 | 293.97 | 294.12 | 294.43 |
| $CH_3CN$ | C1s_CN | 292.60 | 296.17 | 292.71 | 292.67 | 293.01 | 293.61 | 295.93 | 293.55 | 293.76 | 293.98 | 294.28 |
| $C_2H_5NO_2$ | O1s_OH | 540.20 | 544.14 | 540.40 | 540.79 | 540.69 | 541.33 | 543.64 | 541.48 | 541.96 | 541.82 | 542.34 |
| $C_2H_5NO_2$ | O1s_C=O | 538.40 | 542.61 | 538.15 | 539.13 | 538.87 | 539.57 | 542.05 | 539.73 | 540.13 | 539.99 | 540.42 |
| $C_2H_5NO_2$ | N1s | 405.40 | 409.21 | 405.09 | 405.57 | 405.82 | 406.41 | 408.82 | 406.60 | 407.02 | 406.95 | 407.44 |
| $C_2H_5NO_2$ | C1s_COOH | 295.20 | 299.36 | 294.54 | 294.58 | 295.44 | 295.82 | 299.00 | 295.83 | 295.96 | 296.42 | 296.66 |
| $C_2H_5NO_2$ | C1s_CH2 | 292.30 | 296.08 | 291.90 | 292.19 | 292.69 | 293.13 | 295.74 | 293.27 | 293.49 | 293.70 | 294.01 |

**Table S8:** Continued

| formula | core level | Ref | $G_{RSc}W_0$ HF | BLYP | PBE | B3LYP | PBE0 | $G_{RSc}W_{RSc}$ HF | BLYP | PBE | B3LYP | PBE0 |
|---|---|---|---|---|---|---|---|---|---|---|---|---|
| $C_5H_5N$ | N1s | 404.82 | 408.83 | 404.71 | 405.46 | 405.58 | 406.13 | 408.44 | 406.01 | 406.57 | 406.42 | 407.07 |
| $C_4H_4NH$ | N1s | 406.18 | 410.06 | 406.21 | 406.64 | 406.92 | 407.41 | 409.60 | 407.42 | 407.91 | 407.81 | 408.31 |
| $C_6H_5NH_2$ | N1s | 405.31 | 409.17 | 405.38 | 405.82 | 405.88 | 406.51 | 408.72 | 406.55 | 406.98 | 406.86 | 407.36 |
| $CO(NH_2)_2$ | O1s | 537.19 | 541.02 | 537.02 | 538.59 | 537.94 | 538.51 | 540.49 | 538.54 | 539.00 | 538.84 | 539.38 |
| $CO(NH_2)_2$ | N1s | 406.09 | 409.96 | 406.01 | 406.22 | 406.49 | 407.14 | 409.56 | 407.23 | 407.65 | 407.60 | 408.08 |
| $CO(NH_2)_2$ | C1s | 294.84 | 299.09 | 294.18 | 294.22 | 295.13 | 295.52 | 298.78 | 295.52 | 295.63 | 296.12 | 296.37 |
| $CH_3NH_2$ | N1s | 405.17 | 408.80 | 405.05 | 405.35 | 405.50 | 406.11 | 408.46 | 406.32 | 406.74 | 406.63 | 407.12 |
| $C_6H_5NO_2$ | O1s | 538.63 | 543.43 | 539.41 | 539.46 | 539.80 | 540.40 | 542.64 | 540.39 | 540.87 | 540.83 | 541.36 |
| $C_6H_5NO_2$ | N1s | 411.60 | 417.31 | 411.16 | 411.64 | 412.56 | 413.07 | 416.63 | 412.68 | 413.12 | 413.48 | 414.03 |
| $C_6H_5NO_2$ | C1s_C1 | 292.08 | 296.21 | 292.04 | 292.27 | 292.94 | 293.24 | 295.80 | 293.22 | 293.53 | 293.69 | 294.02 |
| $C_6H_5NO_2$ | C1s_C234 | 291.13 | 295.34 | 291.19 | 291.44 | 292.01 | 292.43 | 294.94 | 292.39 | 292.67 | 292.82 | 293.16 |
| $C_6H_6$ | C1s | 290.38 | 294.22 | 290.43 | 290.77 | 291.12 | 291.54 | 293.91 | 291.58 | 291.84 | 291.96 | 292.31 |
| $C_8H_6$ | C1s_C3 | 290.88 | 294.96 | 291.04 | 291.30 | 291.83 | 292.25 | 294.57 | 292.19 | 292.50 | 292.59 | 292.99 |
| $C_8H_6$ | C1s_C2 | 290.55 | 294.45 | 290.50 | 290.76 | 291.26 | 291.74 | 294.09 | 291.66 | 291.96 | 292.08 | 292.43 |
| $C_8H_6$ | C1s_C456 | 290.16 | 294.43 | 290.63 | 290.86 | 291.40 | 291.74 | 294.10 | 291.71 | 292.03 | 292.15 | 292.50 |
| $C_8H_6$ | C1s_C1 | 289.75 | 294.21 | 290.51 | 290.56 | 290.98 | 291.39 | 293.86 | 291.41 | 291.67 | 291.81 | 292.13 |

# 4 Dipole Moments of Small Molecules Obtained from Different *GW* Methods

**Table S9:** Dipole Moments of LiH, HF, LiF and CO obtained from DFT and $G_0W_0$ with HF, BLYP, PBE, B3LYP and PBE0. Reference values were taken from Ref. S4. The def2-TZVPP basis set was used. All values in Debye.

| | Ref | DFT HF | BLYP | PBE | B3LYP | PBE0 | $G_0W_0$ HF | BLYP | PBE | B3LYP | PBE0 |
|---|---|---|---|---|---|---|---|---|---|---|---|
| LiH | 5.88 | 6.02 | 5.56 | 5.60 | 5.71 | 5.76 | 6.10 | 5.39 | 5.49 | 5.54 | 5.78 |
| HF | 1.82 | 1.95 | 1.80 | 1.80 | 1.85 | 1.85 | 1.63 | 1.78 | 1.81 | 1.69 | 1.78 |
| LiF | 6.28 | 6.49 | 5.95 | 5.97 | 6.11 | 6.16 | 6.38 | 6.08 | 6.04 | 6.21 | 6.28 |
| CO | 0.11 | 0.30 | 0.17 | 0.21 | 0.07 | 0.08 | 0.18 | 0.51 | 0.47 | 0.00 | 0.22 |

**Table S10:** Dipole Moments of LiH, HF, LiF and CO obtained from $G_{\mathrm{RS}}W_0$ and $G_{\mathrm{RS}}W_{\mathrm{RS}}$ with HF, BLYP, PBE, B3LYP and PBE0. Reference values were taken from Ref. S4. The def2-TZVPP basis set was used. All values in Debye.

| | | $G_{\mathrm{RS}}W_0$ | | | | | $G_{\mathrm{RS}}W_{\mathrm{RS}}$ | | | | |
|---|---|---|---|---|---|---|---|---|---|---|---|
| | Ref | HF | BLYP | PBE | B3LYP | PBE0 | HF | BLYP | PBE | B3LYP | PBE0 |
| LiH | 5.88 | 6.10 | 5.58 | 5.59 | 5.48 | 5.56 | 6.10 | 5.74 | 5.75 | 5.77 | 5.57 |
| HF | 1.82 | 1.63 | 1.79 | 1.83 | 1.77 | 1.83 | 1.63 | 1.91 | 1.91 | 1.85 | 1.87 |
| LiF | 6.28 | 6.38 | 6.25 | 6.14 | 6.19 | 6.27 | 6.38 | 6.19 | 6.18 | 6.19 | 6.40 |
| CO | 0.11 | 0.18 | 0.27 | 0.16 | 0.48 | 0.36 | 0.18 | 0.01 | 0.00 | 0.10 | 0.06 |

**Table S11:** Dipole Moments of LiH, HF, LiF and CO obtained from $G_{\mathrm{RSc}}W_0$ and $G_{\mathrm{RSc}}W_{\mathrm{RSc}}$ with HF, BLYP, PBE, B3LYP and PBE0. Reference values were taken from Ref. S4. The def2-TZVPP basis set was used. All values in Debye.

| | | $G_{\mathrm{RSc}}W_0$ | | | | | $G_{\mathrm{RSc}}W_{\mathrm{RSc}}$ | | | | |
|---|---|---|---|---|---|---|---|---|---|---|---|
| | Ref | HF | BLYP | PBE | B3LYP | PBE0 | HF | BLYP | PBE | B3LYP | PBE0 |
| LiH | 5.88 | 5.71 | 5.58 | 5.62 | 5.66 | 5.70 | 5.78 | 5.75 | 5.77 | 5.83 | 5.85 |
| HF | 1.82 | 1.78 | 1.82 | 1.80 | 1.83 | 1.80 | 1.81 | 1.79 | 1.89 | 1.77 | 1.80 |
| LiF | 6.28 | 6.34 | 6.09 | 6.08 | 6.18 | 6.22 | 6.29 | 6.20 | 6.16 | 6.51 | 6.14 |
| CO | 0.11 | 0.20 | 0.28 | 0.33 | 0.26 | 0.27 | 0.22 | 0.05 | 0.00 | 0.08 | 0.00 |

# 5 Comparisons of Different RSc Schemes in $G_{\mathrm{RSc}}W_{\mathrm{RSc}}$

**Table S12:** Ionization potentials of the GW100 set[S2] obtained from $G_{\mathrm{RSc}}W_{\mathrm{RSc}}$@B3LYP using three schemes to add the correlation correction. The def2-TZVPP basis set was used. Systems containing Xe, Rb, I, Ag and Cu were excluded because of the convergence problem. All values in eV.

| | | $G_{\mathrm{RSc}}W_{\mathrm{RSc}}$@B3LYP | | |
|---|---|---|---|---|
| name | formula | a | b | c |
| helium | He | 24.64 | 24.62 | 24.62 |
| neon | Ne | 21.62 | 21.58 | 21.58 |
| argon | Ar | 15.54 | 15.56 | 15.56 |
| krypton | Kr | 13.81 | 13.80 | 13.78 |
| hydrogen | $H_2$ | 16.54 | 16.52 | 16.52 |
| lithium dimer | $Li_2$ | 5.31 | 5.31 | 5.31 |
| sodium dimer | $Na_2$ | 5.00 | 5.01 | 5.00 |

**Table S12:** Continued

| name | formula | $G_{RSc}W_{RSc}$@B3LYP | | |
|---|---|---|---|---|
| | | a | b | c |
| sodium tetramer | $Na_4$ | 4.21 | 4.21 | 4.21 |
| sodium hexamer | $Na_6$ | 4.39 | 4.38 | 4.38 |
| potassium dimer | $K_2$ | 4.04 | 4.04 | 4.03 |
| nitrogen | $N_2$ | 15.81 | 15.80 | 15.79 |
| phosphorus dimer | $P_2$ | 10.35 | 10.34 | 10.33 |
| arsenic dimer | $As_2$ | 9.46 | 9.47 | 9.47 |
| fluorine | $F_2$ | 16.08 | 16.07 | 16.07 |
| chlorine | $Cl_2$ | 11.49 | 11.48 | 11.47 |
| bromine | $Br_2$ | 10.45 | 10.43 | 10.42 |
| methane | $CH_4$ | 14.62 | 14.59 | 14.59 |
| ethane | $C_2H_6$ | 12.99 | 12.97 | 12.97 |
| propane | $C_3H_8$ | 12.43 | 12.40 | 12.40 |
| butane | $C_4H_{10}$ | 12.12 | 12.10 | 12.10 |
| ethylene | $C_2H_4$ | 10.63 | 10.62 | 10.61 |
| ethyn | $C_2H_2$ | 11.42 | 11.40 | 11.40 |
| tetracarbon | $C_4$ | 11.32 | 11.30 | 11.30 |
| cyclopropane | $C_3H_6$ | 11.04 | 11.01 | 11.01 |
| benzene | $C_6H_6$ | 9.30 | 9.28 | 9.28 |
| cyclooctatetraene | $C_8H_8$ | 8.38 | 8.36 | 8.35 |
| cyclopentadiene | $C_5H_6$ | 8.65 | 8.63 | 8.63 |
| vinyl fluoride | $C_2H_3F$ | 10.56 | 10.54 | 10.54 |
| vinyl chloride | $C_2H_3Cl$ | 10.09 | 10.07 | 10.07 |
| vinyl bromide | $C_2H_3Br$ | 9.20 | 9.19 | 9.19 |
| tetrafluoromethane | $CF_4$ | 16.53 | 16.48 | 16.49 |
| tetrachloromethane | $CCl_4$ | 11.61 | 11.58 | 11.58 |
| tetrabromomethane | $CBr_4$ | | 10.33 | 10.33 |
| silane | $SiH_4$ | 13.04 | 13.02 | 13.02 |
| germane | $GeH_4$ | 12.64 | 12.63 | 12.63 |
| disilane | $Si_2H_6$ | 10.78 | 10.76 | 10.76 |
| pentasilane | $Si_5H_{12}$ | 9.39 | 9.37 | 9.37 |
| lithium hydride | LiH | 8.19 | 8.17 | 8.16 |
| potassium hydride | KH | 6.32 | 6.27 | 6.28 |

**Table S12:** Continued

| | | $G_{RSc}W_{RSc}$@B3LYP | | |
|---|---|---|---|---|
| name | formula | a | b | c |
| borane | $BH_3$ | 13.54 | 13.53 | 13.53 |
| diborane | $B_2H_6$ | 12.57 | 12.55 | 12.55 |
| ammonia | $NH_3$ | 11.02 | 11.00 | 11.00 |
| hydrazoic acid | $HN_3$ | 10.78 | 10.75 | 10.75 |
| phosphine | $PH_3$ | 10.63 | 10.62 | 10.61 |
| arsine | $AsH_3$ | 10.39 | 10.38 | 10.38 |
| hydrogen sulfide | $SH_2$ | 10.36 | 10.34 | 10.33 |
| hydrogen fluoride | FH | 16.29 | 16.26 | 16.26 |
| hydrogen chloride | ClH | 12.62 | 12.61 | 12.61 |
| lithium fluoride | LiF | 11.60 | 11.55 | 11.55 |
| magnesium fluoride | $F_2Mg$ | 13.99 | 13.93 | 13.93 |
| titanium tetrafluoride | $TiF_4$ | 15.64 | | |
| aluminum fluoride | $AlF_3$ | 15.58 | 15.52 | 15.53 |
| boron monofluoride | BF | 11.08 | 11.07 | 11.07 |
| sulfur tetrafluoride | $SF_4$ | 12.80 | 12.77 | 12.77 |
| potassium bromide | BrK | 8.13 | 8.09 | 8.09 |
| gallium monochloride | GaCl | 9.72 | 9.72 | 9.72 |
| sodium chloride | NaCl | 9.20 | 9.16 | 9.16 |
| magnesium chloride | $MgCl_2$ | 11.73 | 11.70 | 11.70 |
| boron nitride | BN | 11.82 | 11.80 | 11.79 |
| hydrogen cyanide | NCH | 13.72 | 13.70 | 13.69 |
| phosphorus mononitr | PN | 11.92 | 11.94 | 11.94 |
| hydrazine | $H_2NNH_2$ | 9.93 | 9.90 | 9.91 |
| formaldehyde | $H_2CO$ | 11.12 | 11.09 | 11.10 |
| methanol | $CH_4O$ | 11.31 | 11.28 | 11.29 |
| ethanol | $C_2H_6O$ | 10.97 | 10.93 | 10.94 |
| acetaldehyde | $C_2H_4O$ | 10.46 | 10.42 | 10.43 |
| ethoxy ethane | $C_4H_{10}O$ | 10.13 | 10.09 | 10.10 |
| formic acid | $CH_2O_2$ | 11.68 | 11.64 | 11.65 |
| hydrogen peroxide | HOOH | 11.83 | 11.79 | 11.80 |
| water | $H_2O$ | 12.80 | 12.77 | 12.78 |
| carbon dioxide | $CO_2$ | 13.91 | 13.87 | 13.87 |

**Table S12:** Continued

| name | formula | $G_{\mathrm{RSc}}W_{\mathrm{RSc}}$@B3LYP | | |
|---|---|---|---|---|
| | | a | b | c |
| carbon disulfide | $CS_2$ | 9.99 | 9.97 | 9.97 |
| carbon oxide sulfide | OCS | 11.21 | 11.19 | 11.19 |
| carbon oxide selenide | OCSe | 10.38 | 10.36 | 10.35 |
| carbon monoxide | CO | 14.42 | 14.39 | 14.38 |
| ozone | $O_3$ | 13.00 | 13.01 | 13.01 |
| sulfur dioxide | $SO_2$ | 12.46 | 12.44 | 12.44 |
| beryllium monoxide | BeO | 10.23 | 10.18 | 10.18 |
| magnesium monoxide | MgO | 8.19 | 8.25 | 8.26 |
| toluene | $C_7H_8$ | 8.93 | 8.91 | 8.91 |
| ethylbenzene | $C_8H_{10}$ | 8.89 | 8.87 | 8.87 |
| hexafluorobenzene | $C_6F_6$ | 10.01 | 9.98 | 9.99 |
| phenol | $C_6H_5OH$ | 8.71 | 8.69 | 8.69 |
| aniline | $C_6H_5NH_2$ | 8.02 | 8.00 | 8.00 |
| pyridine | $C_5H_5N$ | 9.79 | 9.88 | 9.88 |
| guanine | $C_5H_5N_5O$ | 8.04 | 8.01 | 8.01 |
| adenine | $C_5H_5N_5O$ | 8.34 | 8.30 | 8.30 |
| cytosine | $C_4H_5N_3O$ | 8.85 | 8.81 | 8.82 |
| thymine | $C_5H_6N_2O_2$ | 9.18 | 9.15 | 9.15 |
| uracil | $C_4H_4N_2O_2$ | 9.58 | 9.55 | 9.55 |
| urea | $CH_4N_2O$ | 10.27 | 10.23 | 10.26 |

# 6 Comparison of Using RSc Orbitals and KS Orbitals in $G_{\mathrm{RSc}}W_{\mathrm{RSc}}$

**Table S13:** Ionization potentials of the GW100 set[S2] obtained from $G_{\mathrm{RSc}}W_{\mathrm{RSc}}$ using KS orbitals and using RSc orbitals. The def2-TZVPP basis set was used. Systems containing Xe, Rb, I, Ag and Cu were excluded because of the convergence problem. All values in eV.

| name | formula | $G_{\mathrm{RSc}}W_{\mathrm{RSc}}$@PBE | | $G_{\mathrm{RSc}}W_{\mathrm{RSc}}$@B3LYP | |
|---|---|---|---|---|---|
| | | KS orbital | RSc orbital | KS orbital | RSc orbital |
| helium | He | 24.69 | 24.66 | 24.64 | 24.62 |
| neon | Ne | 21.78 | 21.74 | 21.62 | 21.58 |
| argon | Ar | 15.59 | 15.56 | 15.54 | 15.56 |

**Table S13:** Continued

| name | formula | $G_{RSc}W_{RSc}$@PBE | | $G_{RSc}W_{RSc}$@B3LYP | |
|---|---|---|---|---|---|
| | | KS orbital | RSc orbital | KS orbital | RSc orbital |
| krypton | Kr | 13.81 | 13.81 | 13.81 | 13.80 |
| hydrogen | $H_2$ | 16.56 | 16.54 | 16.54 | 16.52 |
| lithium dimer | $Li_2$ | 5.35 | 5.35 | 5.31 | 5.31 |
| sodium dimer | $Na_2$ | 5.04 | 5.04 | 5.00 | 5.00 |
| sodium tetramer | $Na_4$ | 4.23 | 4.23 | 4.21 | 4.21 |
| sodium hexamer | $Na_6$ | 4.40 | 4.40 | 4.39 | 4.38 |
| potassium dimer | $K_2$ | 4.04 | 4.05 | 4.04 | 4.04 |
| nitrogen | $N_2$ | 15.78 | 15.74 | 15.81 | 15.79 |
| phosphorus dimer | $P_2$ | 10.33 | 10.32 | 10.35 | 10.34 |
| arsenic dimer | $As_2$ | 9.45 | 9.46 | 9.46 | 9.47 |
| fluorine | $F_2$ | 16.19 | 16.17 | 16.08 | 16.06 |
| chlorine | $Cl_2$ | 11.48 | 11.46 | 11.49 | 11.48 |
| bromine | $Br_2$ | 10.44 | 10.44 | 10.45 | 10.43 |
| methane | $CH_4$ | 14.60 | 14.57 | 14.62 | 14.59 |
| ethane | $C_2H_6$ | 12.96 | 12.93 | 12.99 | 12.97 |
| propane | $C_3H_8$ | 12.39 | 12.36 | 12.43 | 12.40 |
| butane | $C_4H_{10}$ | 12.09 | 12.06 | 12.12 | 12.10 |
| ethylene | $C_2H_4$ | 10.61 | 10.60 | 10.63 | 10.62 |
| ethyn | $C_2H_2$ | 11.41 | 11.39 | 11.42 | 11.40 |
| tetracarbon | $C_4$ | 11.43 | 11.40 | 11.32 | 11.30 |
| cyclopropane | $C_3H_6$ | 11.01 | 10.98 | 11.04 | 11.01 |
| benzene | $C_6H_6$ | 9.28 | 9.25 | 9.30 | 9.29 |
| cyclooctatetraene | $C_8H_8$ | 8.32 | 8.29 | 8.38 | 8.36 |
| cyclopentadiene | $C_5H_6$ | 8.61 | 8.59 | 8.65 | 8.64 |
| vinyl fluoride | $C_2H_3F$ | 10.55 | 10.53 | 10.56 | 10.54 |
| vinyl chloride | $C_2H_3Cl$ | 10.05 | 10.03 | 10.09 | 10.07 |
| vinyl bromide | $C_2H_3Br$ | 9.16 | 9.15 | 9.20 | 9.18 |
| tetrafluoromethane | $CF_4$ | 16.57 | 16.50 | 16.53 | 16.48 |
| tetrachloromethane | $CCl_4$ | 11.56 | 11.52 | 11.61 | 11.58 |
| tetrabromomethane | $CBr_4$ | 10.30 | 10.29 | | 10.33 |
| silane | $SiH_4$ | 13.00 | 12.98 | 13.04 | 13.03 |
| germane | $GeH_4$ | 12.60 | 12.59 | 12.64 | 12.63 |

**Table S13:** Continued

| name | formula | $G_{\mathrm{RSc}}W_{\mathrm{RSc}}$@PBE | | $G_{\mathrm{RSc}}W_{\mathrm{RSc}}$@B3LYP | |
|---|---|---|---|---|---|
| | | KS orbital | RSc orbital | KS orbital | RSc orbital |
| disilane | $Si_2H_6$ | 10.68 | 10.65 | 10.78 | 10.76 |
| pentasilane | $Si_5H_{12}$ | 9.25 | 9.23 | 9.39 | 9.37 |
| lithium hydride | LiH | 8.25 | 8.23 | 8.19 | 8.17 |
| potassium hydride | KH | 6.41 | 6.35 | 6.32 | 6.28 |
| borane | $BH_3$ | 13.53 | 13.51 | 13.54 | 13.53 |
| diborane | $B_2H_6$ | 12.51 | 12.48 | 12.57 | 12.55 |
| ammonia | $NH_3$ | 11.07 | 11.05 | 11.02 | 11.00 |
| hydrazoic acid | $HN_3$ | 10.77 | 10.74 | 10.78 | 10.76 |
| phosphine | $PH_3$ | 10.59 | 10.57 | 10.63 | 10.62 |
| arsine | $AsH_3$ | 10.36 | 10.35 | 10.39 | 10.38 |
| hydrogen sulfide | $SH_2$ | 10.34 | 10.32 | 10.36 | 10.34 |
| hydrogen fluoride | FH | 16.46 | 16.41 | 16.29 | 16.26 |
| hydrogen chloride | ClH | 12.65 | 12.62 | 12.62 | 12.61 |
| lithium fluoride | LiF | 11.86 | 11.76 | 11.60 | 11.55 |
| magnesium fluoride | $F_2Mg$ | 14.21 | 14.13 | 13.99 | 13.93 |
| titanium tetrafluoride | $TiF_4$ | 15.70 | | 15.64 | |
| aluminum fluoride | $AlF_3$ | 15.74 | 15.66 | 15.58 | 15.52 |
| boron monofluoride | BF | 11.03 | 11.02 | 11.08 | 11.08 |
| sulfur tetrafluoride | $SF_4$ | 12.76 | 12.72 | 12.80 | 12.77 |
| potassium bromide | BrK | 8.20 | 8.16 | 8.13 | 8.09 |
| gallium monochloride | GaCl | 9.73 | 9.73 | 9.72 | 9.72 |
| sodium chloride | NaCl | 9.29 | 9.23 | 9.20 | 9.16 |
| magnesium chloride | $MgCl_2$ | 11.77 | 11.72 | 11.73 | 11.70 |
| boron nitride | BN | 11.90 | 11.87 | 11.82 | 11.80 |
| hydrogen cyanide | NCH | 13.73 | 13.71 | 13.72 | 13.70 |
| phosphorus mononitr | PN | 11.96 | 11.91 | 11.92 | 11.90 |
| hydrazine | $H_2NNH_2$ | 9.98 | 9.94 | 9.93 | 9.91 |
| formaldehyde | $H_2CO$ | 11.19 | 11.15 | 11.12 | 11.09 |
| methanol | $CH_4O$ | 11.41 | 11.36 | 11.31 | 11.28 |
| ethanol | $C_2H_6O$ | 11.04 | 10.99 | 10.97 | 10.93 |
| acetaldehyde | $C_2H_4O$ | 10.51 | 10.45 | 10.46 | 10.42 |
| ethoxy ethane | $C_4H_{10}O$ | 10.19 | 10.13 | 10.13 | 10.09 |

**Table S13:** Continued

| | | $G_{\mathrm{RSc}}W_{\mathrm{RSc}}$@PBE | | $G_{\mathrm{RSc}}W_{\mathrm{RSc}}$@B3LYP | |
|---|---|---|---|---|---|
| name | formula | KS orbital | RSc orbital | KS orbital | RSc orbital |
| formic acid | $CH_2O_2$ | 11.74 | 11.68 | 11.68 | 11.64 |
| hydrogen peroxide | HOOH | 11.92 | 11.87 | 11.83 | 11.79 |
| water | $H_2O$ | 12.92 | 12.88 | 12.80 | 12.78 |
| carbon dioxide | $CO_2$ | 13.94 | 13.91 | 13.91 | 13.88 |
| carbon disulfide | $CS_2$ | 9.94 | 9.92 | 9.99 | 9.97 |
| carbon oxide sulfide | OCS | 11.17 | 11.15 | 11.21 | 11.19 |
| carbon oxide selenide | OCSe | | 10.33 | 10.38 | 10.36 |
| carbon monoxide | CO | 14.31 | 14.27 | 14.42 | 14.39 |
| ozone | $O_3$ | 12.96 | 12.91 | 13.00 | 12.98 |
| sulfur dioxide | $SO_2$ | 12.44 | 12.40 | 12.46 | 12.43 |
| beryllium monoxide | BeO | 10.54 | 10.48 | 10.23 | 10.18 |
| magnesium monoxide | MgO | 8.54 | 8.42 | 8.19 | 8.11 |
| toluene | $C_7H_8$ | 8.91 | 8.88 | 8.93 | 8.91 |
| ethylbenzene | $C_8H_{10}$ | 8.86 | 8.83 | 8.89 | 8.87 |
| hexafluorobenzene | $C_6F_6$ | 9.89 | 9.85 | 10.01 | 9.99 |
| phenol | $C_6H_5OH$ | 8.73 | 8.70 | 8.71 | 8.69 |
| aniline | $C_6H_5NH_2$ | 8.03 | 8.00 | 8.02 | 8.00 |
| pyridine | $C_5H_5N$ | 9.79 | 9.74 | 9.79 | 9.77 |
| guanine | $C_5H_5N_5O$ | 8.00 | 7.97 | 8.04 | 8.02 |
| adenine | $C_5H_5N_5O$ | 8.31 | 8.28 | 8.34 | 8.32 |
| cytosine | $C_4H_5N_3O$ | 8.85 | 8.81 | 8.85 | 8.82 |
| thymine | $C_5H_6N_2O_2$ | 9.13 | 9.10 | 9.18 | 9.16 |
| uracil | $C_4H_4N_2O_2$ | 10.25 | 10.19 | 9.58 | 9.56 |
| urea | $CH_4N_2O$ | 10.35 | 10.28 | 10.27 | 10.22 |

# References


(S1) Jin, Y.; Su, N. Q.; Yang, W. Renormalized Singles Green's Function for Quasi-Particle Calculations beyond the G0W0 Approximation. *J. Phys. Chem. Lett.* **2019**, *10*, 447–452.

(S2) van Setten, M. J.; Caruso, F.; Sharifzadeh, S.; Ren, X.; Scheffler, M.; Liu, F.; Lischner, J.; Lin, L.; Deslippe, J. R.; Louie, S. G.; Yang, C.; Weigend, F.; Neaton, J. B.; Evers, F.; Rinke, P. GW100: Benchmarking G0W0 for Molecular Systems. *J. Chem.*

*Theory Comput.* **2015**, *11*, 5665–5687.

(S3) Golze, D.; Keller, L.; Rinke, P. Accurate Absolute and Relative Core-Level Binding Energies from GW. *J. Phys. Chem. Lett.* **2020**, *11*, 1840–1847.

(S4) Kaplan, F.; Harding, M. E.; Seiler, C.; Weigend, F.; Evers, F.; van Setten, M. J. Quasi-Particle Self-Consistent GW for Molecules. *J. Chem. Theory Comput.* **2016**, *12*, 2528–2541.
